# Supplementary material for: Ground-state properties of the hydrogen chain: insulator-to-metal transition, dimerization, and magnetic phases
Source: arXiv:1911.01618 ancillary file (2020-07-13)
Supplement: Supplementary file 1 [file si-compressed.pdf]

# Ground-state properties of the hydrogen chain: insulator-to-metal transition, dimerization, and magnetic phases

Mario Motta,[1,2,*] Claudio Genovese,[3,*] Fengjie Ma,[4,*] Zhi-Hao Cui,[2,*] Randy Sawaya,[5,*] Garnet Kin-Lic Chan,[2] Natalia Chepiga,[6] Phillip Helms,[2] Carlos Jiménez-Hoyos,[7] Andrew J. Millis,[8,9] Ushnish Ray,[2] Enrico Ronca,[10] Hao Shi,[8] Sandro Sorella,[3,11] Edwin M. Stoudenmire,[8] Steven R. White,[5] and Shiwei Zhang[8,12,†]

[1] *IBM Almaden Research Center, San Jose, CA 95120, USA*
[2] *Division of Chemistry and Chemical Engineering, California Institute of Technology, Pasadena, CA 91125, USA*
[3] *SISSA – International School for Advanced Studies, Via Bonomea 265, 34136 Trieste, Italy*
[4] *The Center for Advanced Quantum Studies and Department of Physics, Beijing Normal University, Beijing, Beijing 100875, China*
[5] *Department of Physics and Astronomy, University of California, Irvine, CA 92697-4575, USA*
[6] *Institute for Theoretical Physics, University of Amsterdam, Science Park 904 Postbus 94485, 1090 GL Amsterdam, The Netherlands*
[7] *Department of Chemistry, Wesleyan University, Middletown, CT 06459, United States*
[8] *Center for Computational Quantum Physics, Flatiron Institute, New York, NY 10010, USA*
[9] *Department of Physics, Columbia University, New York, NY 10027, USA*
[10] *Max Planck Institute for the Structure and Dynamics of Matter, Luruper Chaussee 149, 22761 Hamburg, Germany*
[11] *Democritos Simulation Center CNR–IOM Istituto Officina dei Materiali, Via Bonomea 265, 34136 Trieste, Italy*
[12] *Department of Physics, College of William and Mary, Williamsburg, VA 23187-8795, USA*

* These authors contributed equally to this work
† szhang@flatironinstitute.org

In this document, we provide additional technical information about the calculations described in the main text, to enable their reproducibility. In the first section, we describe the Hamiltonian studied, and the techniques employed to approach the thermodynamic and infinite basis limits. In the second section, we describe the methodologies used in the present work, computational details, and include additional supporting data.

## I. GENERAL DEFINITIONS

### A. Hamiltonian of the system

A system of $N$ protons at fixed, equally spaced, positions along a line, with $N$ electrons, is described by the Hamiltonian

$$\hat{H} = E_0 - \sum_{i=1}^{N} \frac{\nabla_i^2}{2} + \sum_{i<j=1}^{N} v(\mathbf{r}_i, \mathbf{r}_j) - \sum_{i,a=1}^{N} v(\mathbf{r}_i, \mathbf{R}_a) \quad , \tag{1}$$

with

$$E_0 = \sum_{a<b=1}^{N} \frac{1}{|\mathbf{R}_a - \mathbf{R}_b|} \quad , \quad v(\mathbf{r}, \mathbf{r}') = \frac{1}{|\mathbf{r} - \mathbf{r}'|} \quad . \tag{2}$$

In Eq. (1), $\mathbf{r}_i \in \mathbb{R}^3$, $\mathbf{R}_a = a\,R\,\mathbf{e}_z$, are electronic and nuclear coordinates respectively ($\mathbf{e}_z$ is a unit vector in the $z$ direction), atomic units (Bohr $\mathrm{a_B}$ for lengths, Hartree $\mathrm{E_{Ha}}$ for energies) are used, and $R$ is termed chain bondlength. Eq. (1) describes the neutral H chain with open boundary conditions (OBC). In the present work we studied chains with OBC as well as cells with Born-von-Karman periodic boundary conditions [1], which replaces the Hamiltonian (1) by

$$\hat{H} = E_0 - \sum_{i=1}^{N} \frac{\nabla_i^2}{2} + \sum_{i<j=1}^{N} v'(\mathbf{r}_i, \mathbf{r}_j) + \sum_{i=1}^{N} V_{ext}(\mathbf{r}_i) \quad , \tag{3}$$

an operator acting on a space of wave-functions with the boundary conditions

$$\Psi(\dots \mathbf{r}_i + L\,\mathbf{e}_z \dots) = e^{ikL}\,\Psi(\dots \mathbf{r}_i \dots) \ , \ |k| \leq \frac{\pi}{L} \ . \tag{4}$$

One has periodic boundary conditions (PBC) across the cell when $k = 0$.

In Eq. (3), electronic positions lie within a hyper-cubic cell $\mathbf{r} \in \mathcal{C} = [-L, L] \times [-L, L] \times [0, NR]$, where $L$ is a very large transverse length (vacuum), and $NR$ the cell length. The electron-electron interaction $v(\mathbf{r}, \mathbf{r}')$ and external potential $V_{ext}(\mathbf{r})$ are periodic functions, with periodicity dictated by the shape of the supercell, and $V_{ext}$ depends on nuclear positions and can optionally include a non-local pseudo-potential. Finally, $E_0$ is a constant correction arising from the treatment of long-range terms in the Coulomb interactions and pseudopotential.

Many of the methods employed work in a finite basis (see Section I C and others for further discussion). The Hamiltonian projected into an orthogonal basis of $2M$ spin-orbitals can be written in second quantization as

$$\hat{H} = \sum_{pq,\sigma} h_{pq}\,\hat{a}^\dagger_{p\sigma} \hat{a}_{q\sigma} + \frac{1}{2} \sum_{pqrs,\sigma\tau} (pr|qs)\,\hat{a}^\dagger_{p\sigma} \hat{a}^\dagger_{q\tau} \hat{a}_{s\tau} \hat{a}_{r\sigma} \quad , \tag{5}$$

where $\hat{a}^\dagger_{p\sigma}$ ($\hat{a}_{p\sigma}$) destroys (creates) an electron in the orbital $p$ with spin $\sigma$ along the $z$-axis of a suitable reference frame.

As a simplification of the full second-quantized Hamiltonian, in the present work we have also studied the one-band one-dimensional (1D) Hubbard model

$$\hat{H} = - \sum_{\langle ij \rangle,\sigma} \left( \hat{a}^\dagger_{i\sigma} \hat{a}_{j\sigma} + \text{h.c.} \right) + \sum_{i} U\,\hat{a}^\dagger_{i\uparrow} \hat{a}_{i\uparrow} \hat{a}^\dagger_{i\downarrow} \hat{a}_{i\downarrow} \quad , \tag{6}$$

where the summation in the one-body part of the Hamiltonian is performed over nearest neighbors indices $ij = 1 \dots N$ in the topology of the system (straight-line or ring for OBC, PBC respectively), and $U \geq 0$ is a parameter controlling the relative importance of the interaction part of the Hamiltonian.

### B. Size effects

To approach the thermodynamic limit $N \to \infty$, we studied increasingly large chains with OBC or increasingly large cells with PBC. With the latter, we remove part of the size effects by means of the twist-average boundary condition procedure [2]: a mesh $\{k_i\}_{i=1}^{N_k}$ of twist vectors in the first Brillouin zone of the cell, $k \in [-\pi/L, \pi/L]$, is chosen. For every $k_i$ in such mesh, a simulation is conducted, giving access to an approximation for the ground-state wave-function $\Psi_{k_i}$ of the Hamiltonian Eq. (3) with boundary conditions dictated by $k_i$. An observable of interest (such as the ground-state energy) is computed as

$$O_{k_i} = \langle \Psi_{k_i} | \hat{O} | \Psi_{k_i} \rangle \quad , \tag{7}$$

and its average over twists is computed as $O = \frac{1}{N_k} \sum_{i=1}^{N_k} O_{k_i}$. For metallic systems, averaging over twist vectors is especially important and results in faster convergence to the thermodynamic limit than PBC for many properties, without any significant increase in computational cost in stochastic methods [2]. Complete removal of finite-size effects is achieved combining twist-averaging for a cell containing $N$ atoms, and increasing $N$ until the observable of interest has converged or a reliable extrapolation is possible.

### C. Basis sets

Of the methodologies employed in the present work, VMC and DMC operate directly in a continuum basis, where electrons occupy real-space positions $\mathbf{r} \in \mathbb{R}^3$. Finite basis effects in these methods are typically tiny and enter only via the trial wave-function form and the fixed-node approximation (see Sec. II F for details). The other electronic structure methods operate in a finite basis. The basis set error can lead to biases in the results, which can be quantitative or qualitative in nature depending on the observable of interest and the basis used.

In the case of independent-electron methods (such as DFT or Hartree-Fock) it is in practice possible to use large basis sets. These basis sets can for example, be composed of plane waves, Gaussians, or specialized bases such as sliced Gaussian bases that are described in more detail below. The basis set error for mean-field results can thus be controlled reasonably well on the energy scale of interest in the current study (e.g. to significantly better than 1 m$E_h$ per atom). For example, in the planewave DFT calculations (see Sec. II A), convergence with respect to basis error is straightforward to control, and the results are converged for the effective Hamiltonian in which the protons are replaced by a pseudopotential.

For the correlated electronic methods, the basis set error is more problematic both because it is often difficult to use such large basis sets, and because the basis set error typically converges more slowly than it does for independent-electron methods. In modest to large $R$ regimes, we have demonstrated how the basis set error could be removed and the continuum limit achieved in several many-body methods [3]. In the small $R$ metallic regime, this turns out to be more challenging, as discussed in further detail below. It is thus necessary to work with a more compact representation. The correlated methods then either use a smaller basis of the same kind as the mean-field calculations, or project the large mean-field computational basis onto a smaller, specially constructed set. The details of the compact basis construction are reported below for each method. With these restrictions, the basis error in the energy in the correlated methods remains larger than 1 m$E_h$ per atom, sometimes substantially so. However, we only draw conclusions of a qualitative nature that depend on observables that are relatively insensitive to this error. Examples where this is not the case, for example precise occupancies in the metallic phase, are briefly discussed in the main text and illustrated further below.

## II. NUMERICAL METHODS AND RESULTS

In this section, technical information is presented in separate subsections under each method, first for mean-field methods, followed by correlated methods. In each subsection, the method is described, followed by computational details, under "Approach and computational details", which may also include data related to technical details (basis set convergence, size convergence, etc). Then in "Additional data" other supplementary results computed by the method, if available, are presented, organized according to the order of the discussion and figures in the main text.

### A. Density functional theory (DFT)

#### 1. *Approach and computational details*

In the present work, the plane-wave basis method and Quantum-ESPRESSO software package [4] were used to perform DFT calculations. Generalized gradient approximations (GGA) of Perdew-Burke-Ernzerhof (PBE) have been adopted for exchange-correlation potential [5]. The multi-projector optimized norm-conserving Vanderbilt pseudopotential [6, 7] was used to model the electron-ion interactions, with the kinetic energy cutoff for wavefunctions fixed at $E_{cut} = 60\,\mathrm{Ry}$. Several other types of exchange-correlation functional, including the local density approximation (LDA) of the Perdew-Zunger formula [8], the Heyd-Scuseria-Ernzerhof (HSE) screened hybrid functional [9, 10], and the Gaussian-Perdew-Burke-Ernzerhof (Gau-PBE) screened hybrid functional [11] were also tested and used for comparison. In order to minimize the interaction between periodic images in the $x$ and $y$ directions (H atoms are placed along the $z$ axis), a large vacuum of length $L = 40\ \mathrm{a}_B$ was imposed in all calculations.

As illustrated in Fig. 1 for a 50-atom supercell at $R = 1.4\,\mathrm{a}_B$, calculations may predict the wrong ground state if the vacuum length $L$ is not large enough.

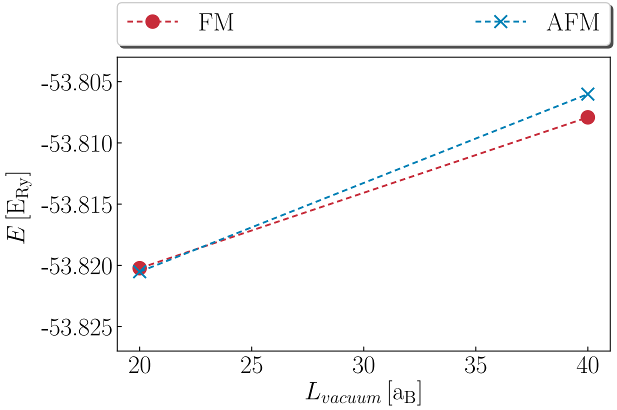


FIG. 1. Effect of increasing the vacuum length $L$ (size of the supercell in directions perpendicular to the chain axis) on DFT-GGA energies, for $N = 50$ atoms, at $R = 1.4\,\mathrm{a}_B$.

#### 2. *Additional data*

The DFT-GGA bands for $R < 1.1\,\mathrm{a_B}$ and $R \geq 1.6\,\mathrm{a}_B$ are shown in Fig. 2. The cells contain $N = 33, 20, 24, 30$ H atoms for $R = 0.7\,\mathrm{a_B}$ to $R = 1.0\,\mathrm{a_B}$, respectively. Cells of $N = 2$ atoms are used for $R \geq 1.6\,\mathrm{a}_B$.

In these regimes, DFT-GGA predicts modulated FM metals and AFM insulators as ground states respectively. Since these systems are overall in AFM order, the band structures of spin-up and spin-down parts are the same. Their energy gaps increase with $R$ in the insulating phase.

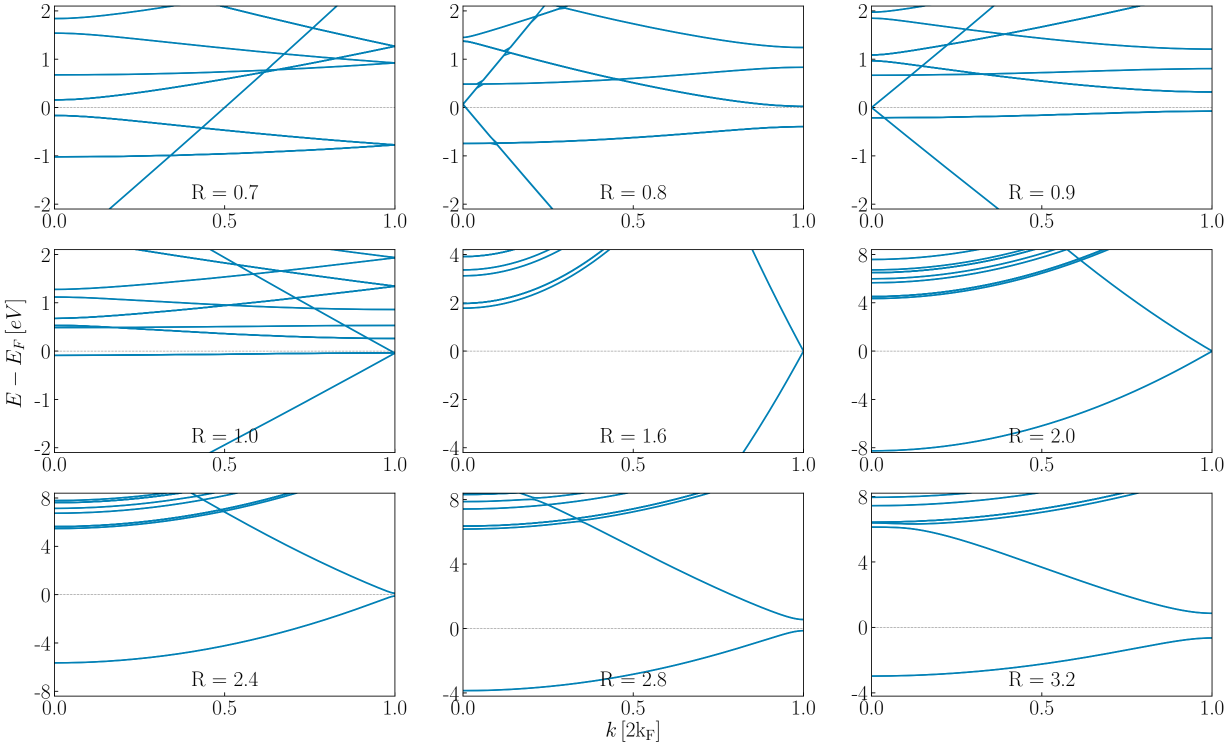


FIG. 2. Top to bottom: DFT-GGA bands for $R < 1.1\,\mathrm{a_B}$ (modulated FM) and $R \geq 1.6\,\mathrm{a}_B$ (AFM insulator). Energies are measured from the Fermi level, in electronvolts (eV), and momenta in units of the Fermi wave-vector of a paramagnetic ideal Fermi gas with density $1/R$.

In Fig. 3, the orbital characters of the DFT-GGA bands, as analyzed by projection onto atomic orbitals, are shown for $R = 0.8$, 1.0, 1.1, 1.6, and $2.0\,\mathrm{a_B}$.

For large $R$ when the system is insulating, the occupied bands consist basically of $1s$ orbitals, as expected. Bands with $2s$ characters have energy slightly lower than bands with $2p_x$ or $2p_y$ characters. However, an inversion of the band order is seen as $R$ decreases, with bands of mostly $2p_x$ or $2p_y$ character becoming lower in energy than the $2s$ one, and thus becoming the first bands to be populated. An insulator-to-metal transition occurs, and the system enters a metallic phase.

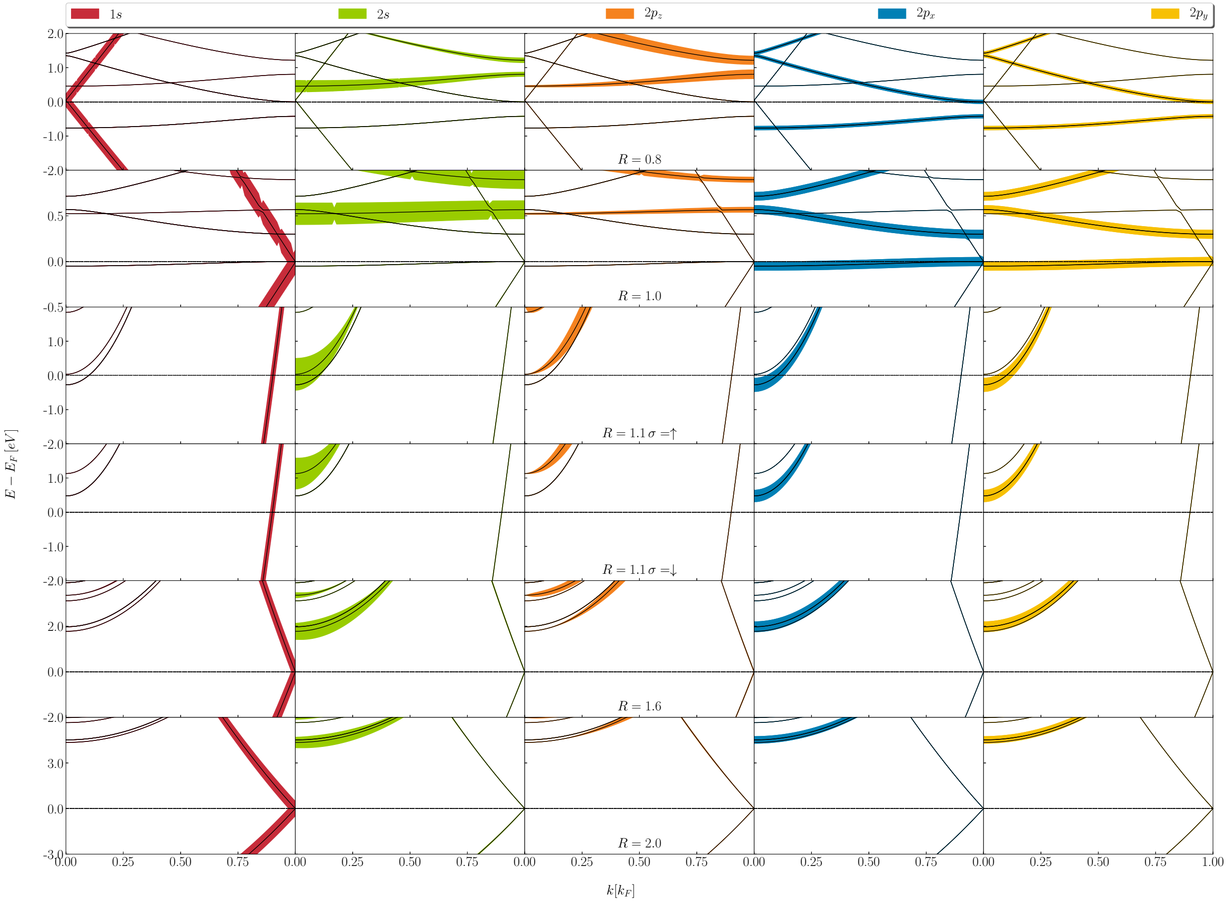


FIG. 3. DFT-GGA bands for $R = 0.8$, $1.0$, $1.1\,\mathrm{a_B}$ (modulated FM) and $R = 1.6$, $2.0\,\mathrm{a}_B$ (AFM insulator). Projections of DFT orbitals onto subspaces spanned by $1s$, $2s$, $2p_z$, $2p_x$, $2p_y$ orbitals are showed (left to right), centered around the energies $E(k)$ of DFT orbitals. The thickness is proportional to the squared amplitude of their projections on the angular-momentum eigenspaces. For $R = 1.1\,\mathrm{a_B}$, spin-up and spin-down bands are shown separately.

In the intermediate regime, for $R$ between $1.1$ and $1.4\,\mathrm{a_B}$, long-range FM order develops in the DFT-GGA ground state. The spin-resolved and orbital-projected bands for $R = 1.2$, $1.3$, and $1.4\,\mathrm{a_B}$ are shown in the top panels of Fig. 4, Fig. 5, and Fig. 6, respectively, using 2-atom supercells.

Bands with $2p_x$ or $2p_y$ characters have lower energy than the $2s$ one, and contribute mostly to the spin polarization and magnetic order. The influence of the exchange-correlation functional on the electronic structure is studied using an efficient hybrid Gau-PBE functional, which goes beyond the standard functionals LDA and GGA. Results are shown in the bottom panels of Fig. 4, Fig. 5, and Fig. 6. The two exchange-correlation functionals give similar results, except that the inversion of $2s$ and $2p_x$ or $2p_y$ happens a little later in the Gau-PBE calculations, with the bands of $2s$ character being lower in energy than the $2p_x$ and $2p_y$ until $R = 1.4\,\mathrm{a_B}$.

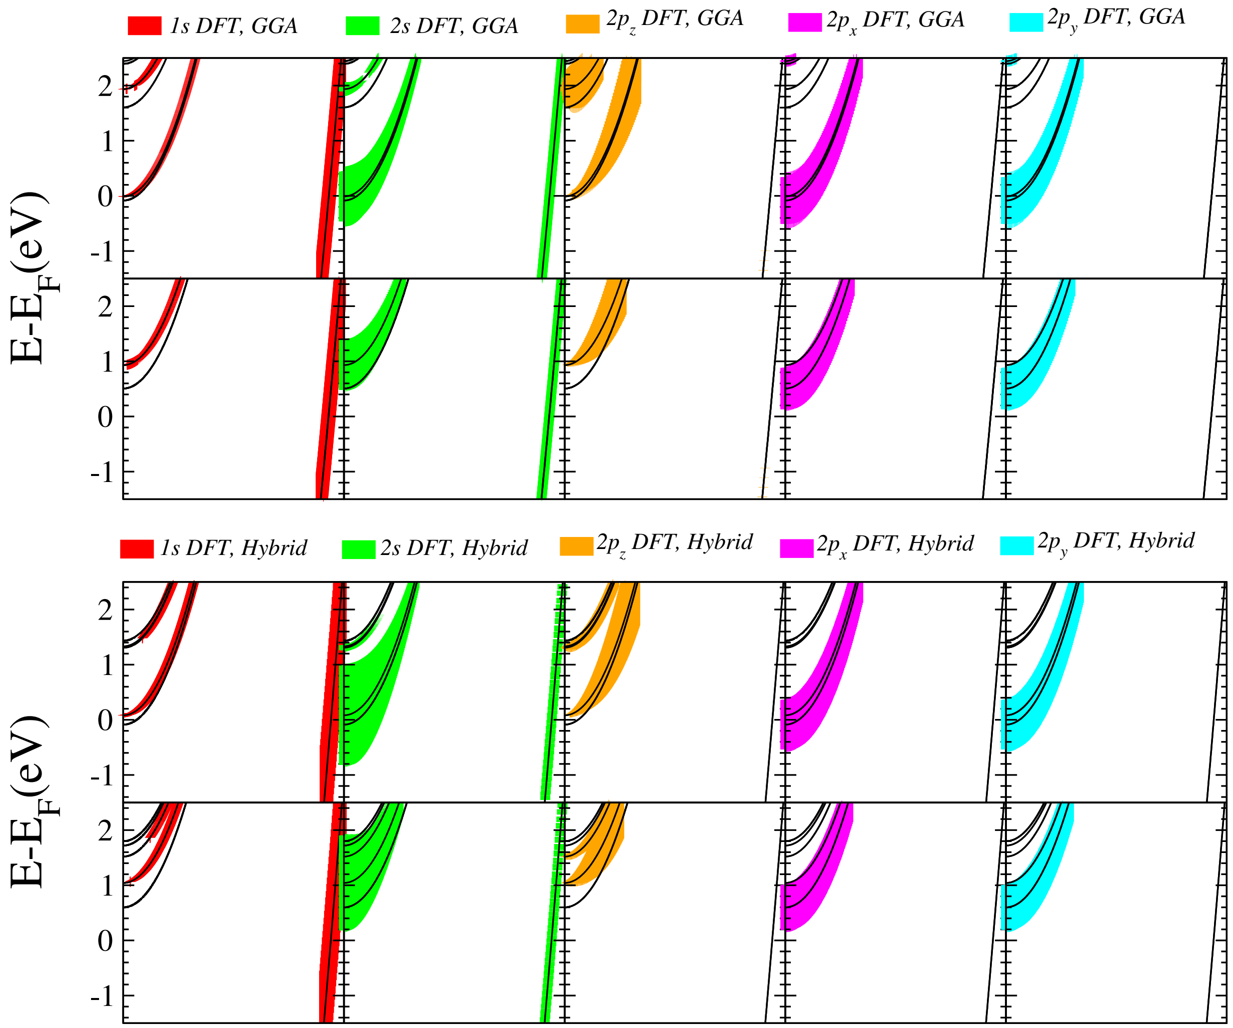


FIG. 4. Spin-resolved and orbital-projected bands for $R = 1.2\mathrm{a_B}$, from DFT-GGA (top) and a hybrid Gau-PBE functional (bottom). Projections of DFT orbitals onto subspaces spanned by $1s$, $2s$, $2p_z$, $2p_x$, $2p_y$ orbitals are shown (left to right), centered around the energies $E(k)$ of DFT orbitals, with thickness proportional the squared amplitude of their projections on the angular-momentum eigenspaces.

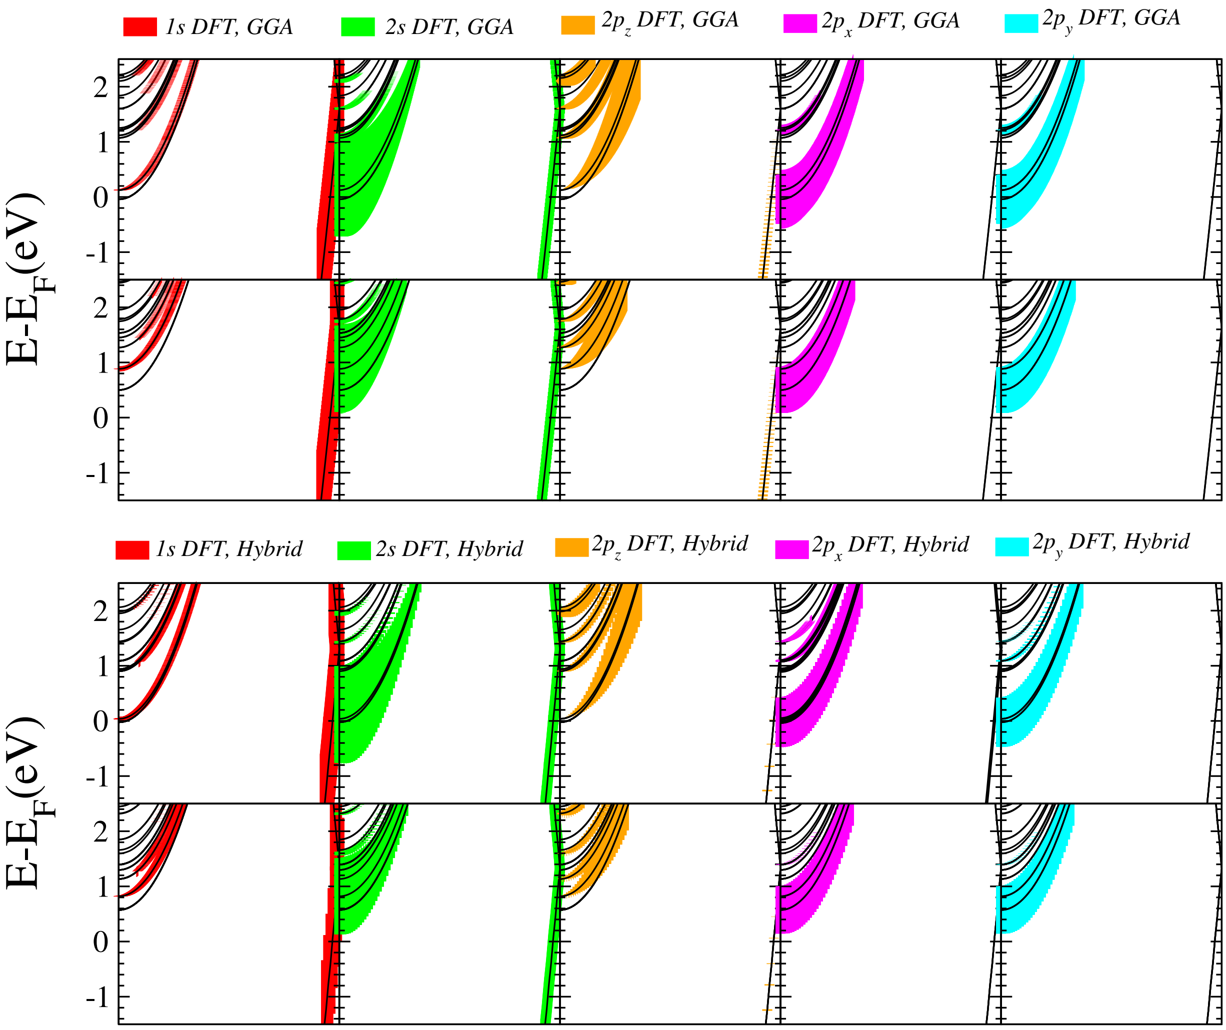


FIG. 5. Similar to Fig. 4, but for $R = 1.3\mathrm{a_B}$.

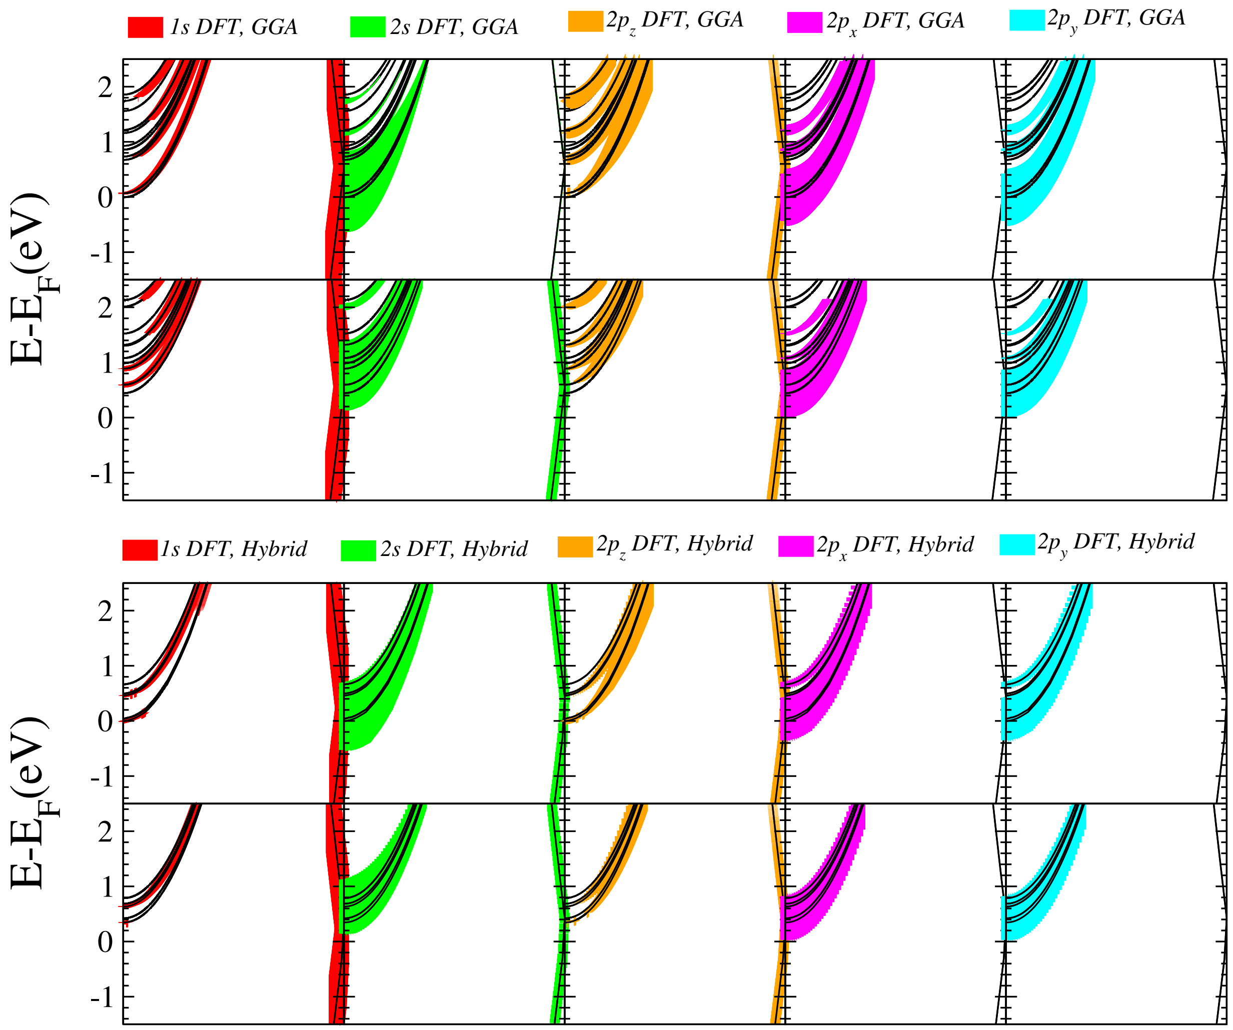


FIG. 6. Similar to Fig. 4, but for $R = 1.4\mathrm{a_B}$.

The magnetic properties of the H chain in the insulating regime, such as the absolute magnetization and charge gap, are shown in Fig. 7. Gaps from two standard LDA and GGA exchange-correlation functionals, and two screened hybrid functionals (HSE and Gau-PBE) are shown. As $R$ increases, both the absolute magnetization and charge gap increase.

GGA, which includes more non-local exchange interactions than LDA, predicts a stronger magnetization, and larger charge gaps. Both functionals tend to underestimate the charge gap, a fact known as the "band gap problem". Hybrid functionals incorporating a portion of exact exchange from Hartree-Fock theory would give more accurate estimates. However, the metal-insulator transition is not sensitive to the exchange-correlation functionals adopted.

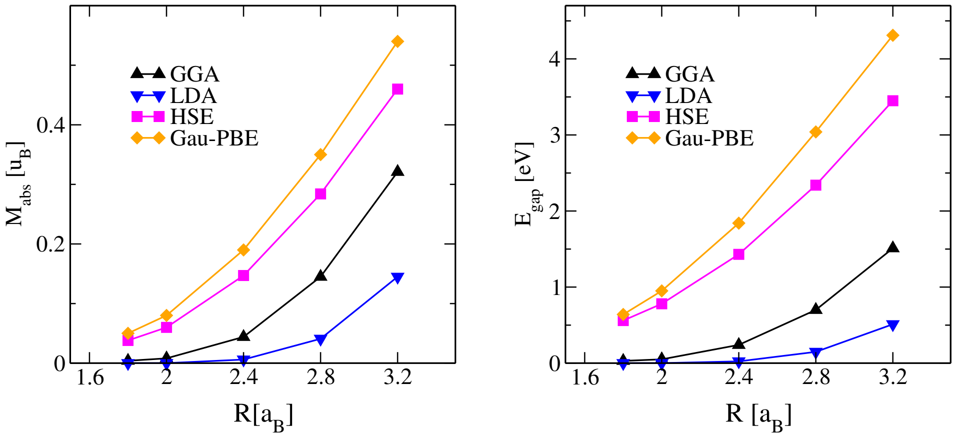


FIG. 7. The absolute magnetization (left) and charge gap (right) as a function of $R$ from GGA, LDA, HSE, and Gau-PBE calculations in the insulating regime.

Figure 8 gives the detailed spin-density computed from DFT-GGA, shown along a plane containing the chain, to illustrate the spin density distributions at $R = 0.7$ to $R = 3.2\,\mathrm{a_B}$. Three types of long-range orders are found. For large $R$ ($R \geq 1.6\,\mathrm{a_B}$), when the systems is insulating, antiferromagnetic order develops, with alternating spin-up and spin-down along the chain. As R decreases, the systems undergoes a metal-insulator transition. As discussed before, the bands of $2p_x$, and $2p_y$ characters become partially occupied and long-range modulated FM domains are formed. In the intermediate regime ($R \geq 1.1\,\mathrm{a_B}$ and $R < 1.6\,\mathrm{a_B}$), the system shows a ferromagnetic order with spin polarization, mostly due to $2p_x$, and $2p_y$ bands. As R further decreases, the modulation of the FM domains become shorter, as shown in the figures for $R = 0.7$ to $R \leq 1.0\,\mathrm{a_B}$.

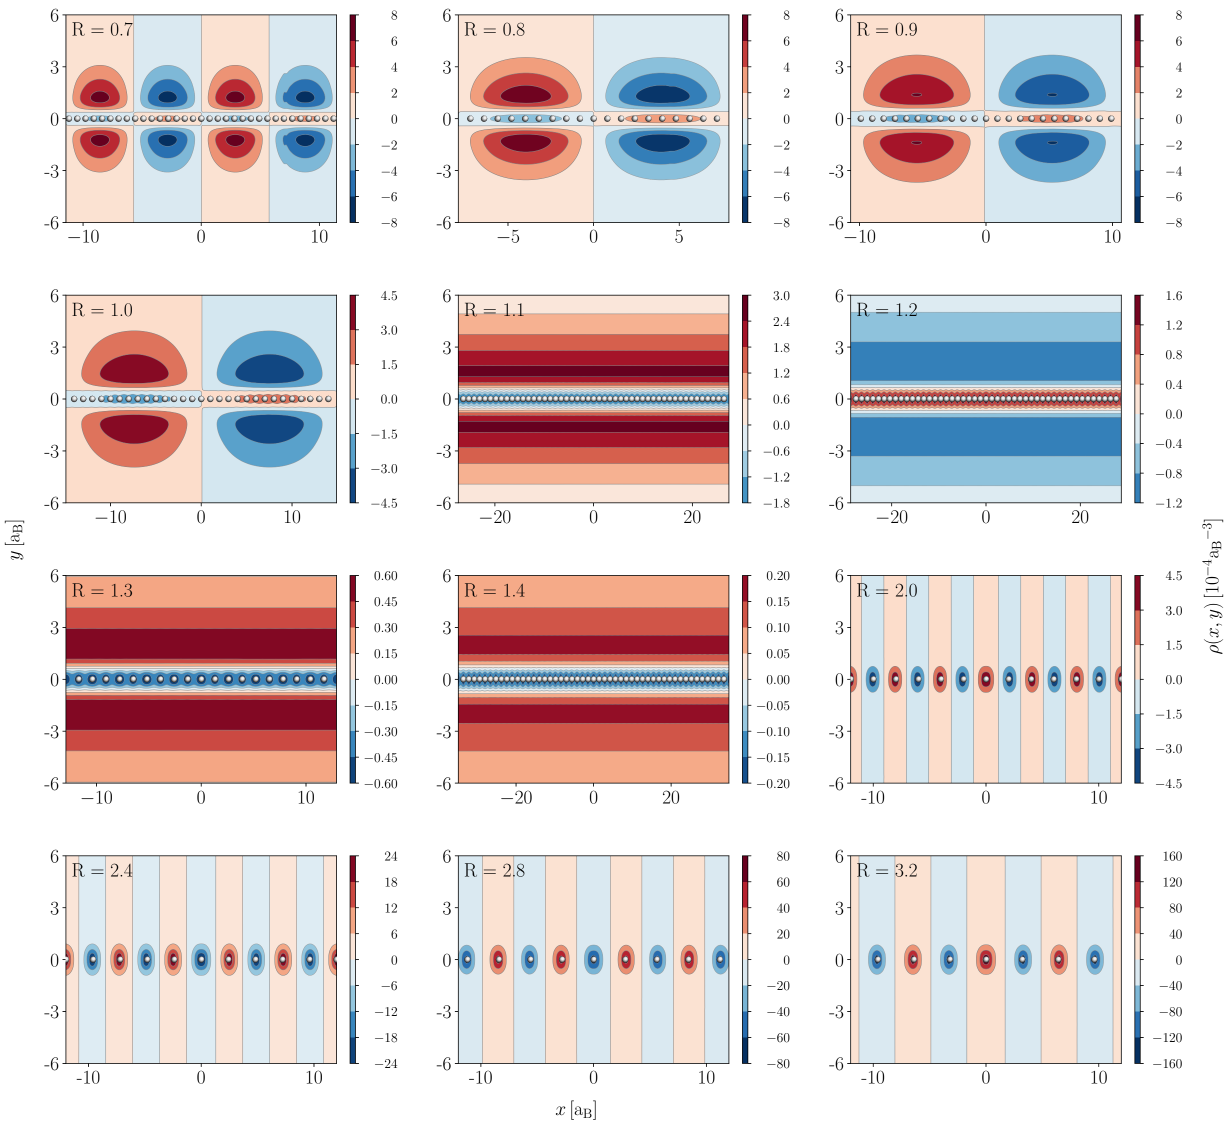

FIG. 8. Spin-density computed from DFT-GGA, shown along a plane containing the chain, to illustrate the spin density distributions at $R = 0.7$ to $R = 3.2\,\mathrm{a_B}$ .

The extrapolation of the dimensionless localization length $D$ at $R = 1.8$, 2.5, and $3.0\,\mathrm{a_B}$ at DFT level is shown in Fig. 9. As mentioned in the main text, the electron localization length $\Lambda$ is related to the complex polarization $Z_N$ by $\Lambda = \frac{\sqrt{D}}{2\pi\rho}$ and $D = -\lim_{N\to\infty} N \log |Z_N|^2$. In localized systems, $\lim_{N\to\infty} |Z_N|^2 = 1$, and $D$ or $\Lambda$ is finite; in metallic systems $\lim_{N\to\infty} |Z_N|^2 = 0$, and $D$ or $\Lambda \to \infty$. For small R, DFT calculations give $|Z_N| = 0$ across a wide range of system sizes N, indicating a metallic ground state. The values of $|Z_N|$ are always larger than 0 for large R, in consistent with the insulating ground state. However, the values of $|Z_N|$ in the insulating phase are sensitive to finite-size effects, as illustrated in the Fig. 9. The closer to $R_{\mathrm{MIT}}$, the slower the corresponding localization length $D$ converges. For example, up to $N = 160$, the values of $D$ are far away from convergence at $R = 1.8\,\mathrm{a_B}$. When $R$ is larger, the convergence becomes much better, as shown as the curve of $R = 2.5\,\mathrm{a_B}$. However, the values of $D$ are still not converged when $N = 160$, which suggests that the correlation length of the MIT $\xi$ is large even at $R \sim 2.5\,\mathrm{a_B}$. For $R = 3.0\,\mathrm{a_B}$, the values of $D$ are almost converged when $N \sim 100$, indicating a strong electron localization.

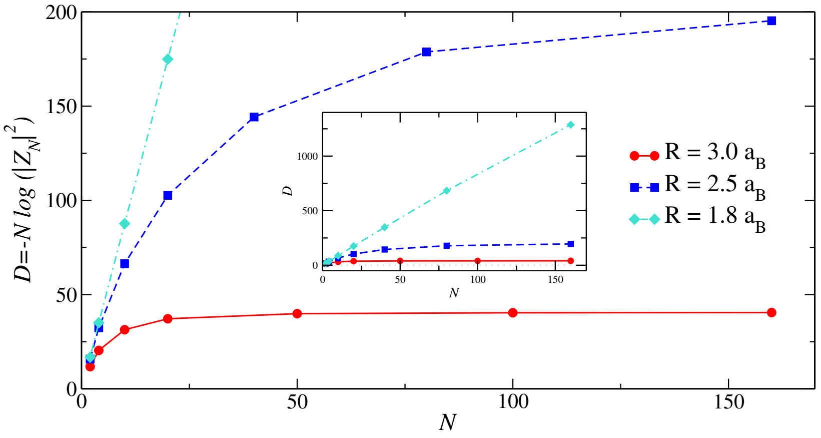


FIG. 9. The extrapolation of the dimensionless localization length $D$ at $R = 1.8$, 2.5, and 3.0 $\mathrm{a_B}$ at DFT level. Inset: zoomed plot of the main figure.

## B. Auxiliary-field quantum Monte Carlo (AFQMC)

### 1. *Approach and computational details*

The auxiliary-field quantum Monte Carlo (AFQMC) estimates the ground-state properties of a many-fermion system by statistically sampling the wave-function $e^{-\beta\hat{H}}|\Psi_I\rangle \propto |\Psi_\beta\rangle \to |\Psi_G\rangle$, where $\Psi_I$ is an initial wave-function, non-orthogonal to the ground state $\Psi_G$ of $\hat{H}$ [12, 13]. For sufficiently large $\beta$, expectation values computed over $\Psi_\beta$ gives ground-state averages. AFQMC projects $\Psi_I$ towards $\Psi_G$ iteratively, writing $e^{-\beta\hat{H}} = (e^{-\Delta\tau\hat{H}})^n$ where $\Delta\tau = \frac{\beta}{n}$ is a small imaginary-time step. The propagator is represented as $e^{-\Delta\tau\hat{H}} = \int d\mathbf{x}\, p(\mathbf{x})\, \hat{B}(\mathbf{x})$, where $\hat{B}(\mathbf{x})$ is a mean-field propagator, of the form of an exponential of one-body operators and depending on the vector $\mathbf{x}$, and $p(\mathbf{x})$ is a probability distribution [14, 15]. This representation maps the original interacting system onto an ensemble of non-interacting systems subject to a fluctuating potential. The imaginary-time projection can be realized as an open-ended random walk over the auxiliary-field (i.e., mean-field potential) configurations [12, 13]. Sampling the trajectories of the random walk leads to a stochastic representation of $\Psi_\beta$ as an ensemble of Slater determinants. For general two-body interactions AFQMC has a sign/phase problem, which is controlled by a phaseless gauge constraint (CP) on the Slater determinants using a trial wave-function $\Psi_T$ [12, 13]. (For Hamiltonians that satisfy certain symmetry properties, e.g. the Hubbard model at half-filling, AFQMC is free of the sign problem). Here, the trial wave-function is typically taken from Hartree-Fock or DFT. The accuracy of the CP AFQMC was extensively benchmarked in both real materials [3] and lattice models [16–18].

For first-principles materials computations, AFQMC can be carried out using either a plane-wave basis and pseudopotentials [12, 19], localized basis sets such as standard Gaussian type orbitals [13], or down-folded Hamiltonians [20]. In this work, we used Gaussian bases to study finite chains with OBC, and down-folded bases to study cells with PBC. For OBC calculations, the two-body matrix elements $(pr|qs)$ are decoupled into rank-3 tensors with the Cholesky decomposition, using a tolerance of $\delta \leq 10^{-5}$ [21]. The total projection time is typically $\beta = 200\,\mathrm{E_{Ry}^{-1}}$, although calculations with higher $\beta$ were performed in some cases. The convergence error from the use of a finite $\beta$ is negligible. Most calculations used $\Delta\tau = 0.005$ or $0.01\,\mathrm{E_{Ry}^{-1}}$, and a population of $N_w \simeq 400$ stochastically sampled Slater determinants. The reported QMC error bars are estimated as one standard deviation statistical errors.

*a. Backpropagation* Observables other than the energies can be computed relying on the back-propagation algorithm [22–24] in the framework of AFQMC, related to the forward walking method in configurational quantum Monte Carlo [25, 26]. The starting point of the BP algorithm is the observation that, for large $n$ and $m$,

$$A \equiv \frac{\langle\Psi_T|e^{-m\Delta\tau\hat{H}}\hat{A}e^{-n\Delta\tau\hat{H}}|\Psi_I\rangle}{\langle\Psi_T|e^{-(m+n)\Delta\tau\hat{H}}|\Psi_I\rangle} \simeq \langle\Psi_G|\hat{A}|\Psi_G\rangle\,. \tag{8}$$

Inserting the stochastic representation of the imaginary-time propagator gives

$$A = \sum_i W_i \frac{\langle\Phi_i|\hat{A}|\Psi_i\rangle}{\langle\Phi_i|\Psi_i\rangle} \quad . \tag{9}$$

Here, $|\Psi_i\rangle$ is a stochastically sampled Slater determinant sampled at imaginary time $n\,\Delta\tau$, $W_i$ its normalized future weight at some time $(n+m)\,\Delta\tau$ and $\langle\Phi_i|$ is obtained back-propagating (i.e. propagating as a bra or linear functional, rather than a ket or vector) $\langle\Psi_T|$ along the segment of the future path of $|\Psi_i\rangle$, sampled during the time interval between $n\,\Delta\tau$ and $(n+m)\,\Delta\tau$ [24].

In this work, we employed the back-propagation algorithm to evaluate the spin-resolved one-body density matrix,

$$\rho_{pq,\sigma} = \langle\Psi_G|\hat{a}^\dagger_{p\sigma}\hat{a}_{q\sigma}|\Psi_G\rangle \quad , \tag{10}$$

the complex polarization measure

$$Z = \langle\Psi_G|e^{i\frac{2\pi}{L}\sum_{pq\sigma} x_{pq}\hat{a}^\dagger_{p\sigma}\hat{a}_{q\sigma}}|\Psi_G\rangle \quad , \tag{11}$$

where $L$ is the length of the simulation cell and $x_{pq}$ the matrix elements of the position operator $\hat{x}$, and the spin structure factor

$$\begin{aligned} S(q) &= \frac{1}{N_w}\left(\langle\Psi_G|\hat{\rho}_s(q)^\dagger\hat{\rho}_s(q)|\Psi_G\rangle - |\langle\Psi_G|\hat{\rho}_s(q)|\Psi_G\rangle|^2\right) \quad , \\ \hat{\rho}_s(q) &= \sum_{pr\sigma}(-1)^\sigma\,\rho_{pr}(q)\,\hat{a}^\dagger_{p\sigma}\hat{a}_{r\sigma} \quad , \end{aligned} \tag{12}$$

where $\rho_{pr}(q)$ are the matrix elements of the density fluctuation operator $\hat{\rho}(q) = e^{iq\hat{x}}$. These quantities can be explicitly evaluated using a combination of Wick's and Thouless's theorems [13]. Indeed, defining the matrices parametrizing the Slater determinants in (9) as $\Phi_i^\sigma$ and $\Psi_i^\sigma$, and their Green's function as

$$G_i^\sigma = \Psi_i^\sigma\left((\Phi_i^\sigma)^\dagger\,\Psi_i^\sigma\right)^{-1}(\Phi_i^\sigma)^\dagger \quad , \tag{13}$$

one has

$$\begin{aligned} \rho_{pq,\sigma} &= \sum_i W_i\,(G_i^\sigma)_{qp} \quad , \\ Z &= \sum_i W_i \prod_\sigma \frac{\det\left((\Phi_i^\sigma)^\dagger\,e^{i\frac{2\pi}{L}x}\Psi_i^\sigma\right)}{\det\left((\Phi_i^\sigma)^\dagger\,\Psi_i^\sigma\right)} \end{aligned} \tag{14}$$

and, in the case of a closed-shell system,

$$S(q) = \sum_{i\sigma}\frac{W_i}{N_w}\,\mathrm{Tr}[\rho^\dagger(q)G_i^\sigma\rho(q) - \rho^\dagger(q)G_i^\sigma\rho(q)G_i^\sigma] \quad . \tag{15}$$

In the infinite basis limit one has $\rho^\dagger(q)\rho(q) = \rho(q)\rho^\dagger(q) = \mathbb{I}$, which does not hold for a finite basis. We alleviate this finite-basis effect by replacing the estimator of the spin structure factor with

$$S(q) = 1 - \sum_{i\sigma}\frac{W_i}{N_w}\,\mathrm{Tr}[\rho^\dagger(q)G_i^\sigma\rho(q)G_i^\sigma] \quad . \tag{16}$$

In Figure 10 we show the AFQMC localization measure as a function of twist vector $k$ for a 40-atom supercell at $R = 1.8\,\mathrm{a_B}$. Localization measure is computed using a back-propagation time of $\beta = 1\mathrm{E_{Ry}}$ and a population of $N_w = 1000$ walkers on average.

*b. Down-folding* Down-folding techniques aim at producing model Hamiltonians that capture emergent correlated physics of interacting systems, by focussing on a relevant low-energy subspace of the original Hilbert space. In correlated systems, the correct effective Hamiltonian is strongly dependent on material-specific properties, motivating the need for general-purpose, accurate and systematic procedures.

In the present work we resorted to a down-folding technique [20, 27] that expresses down-folded Hamiltonians with respect to a truncated basis set of mean-field orbitals of the original system.

The construction of the down-folded Hamiltonian begins with a standard DFT calculation for the target system. This is done using a plane-wave basis with pseudopotentials. Plane-waves are desirable at this stage, because they provide an unbiased representation of the many-body Hamiltonian. We then use the Kohn-Sham (KS) orbitals $\{\chi_i\}_{i=1}^M$ as basis set, tuned to eliminate less physically relevant high-energy virtual states, based on the Kohn-Sham energies $\{\epsilon_i\}_{i=1}^M$. In this work, the KS orbitals used as basis are solved after a self-consistent DFT calculation, adding a potential term in the KS Hamiltonian that confines theresulting orbitals according to the electronic density, so that the high-energy orbitals can be highly diffuse but not unbound.

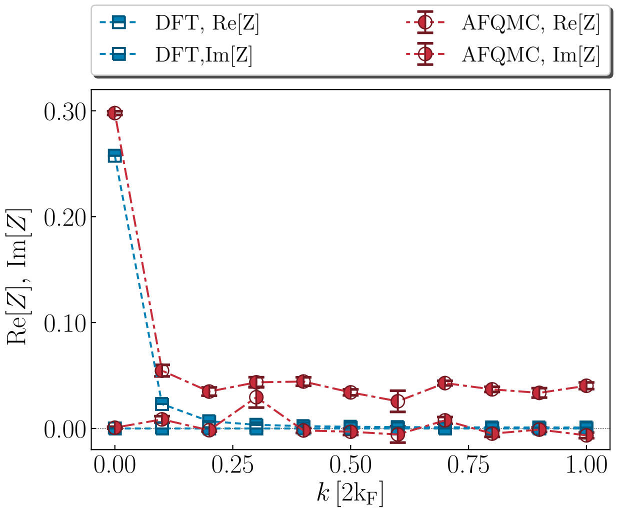


FIG. 10. (color online) Detail of the twist-average procedure for the calculation of Re$[Z]$, Im$[Z]$ for a 40-atom supercell at $R = 1.8\,\mathrm{a_B}$, using AFQMC (red half-filled spheres) and DFT (blue half-filled squares). $k$ is given in units of the Fermi wave-vector $2k_F = \pi/R$ of a paramagnetic 1D ideal Fermi gas with density $1/R$.

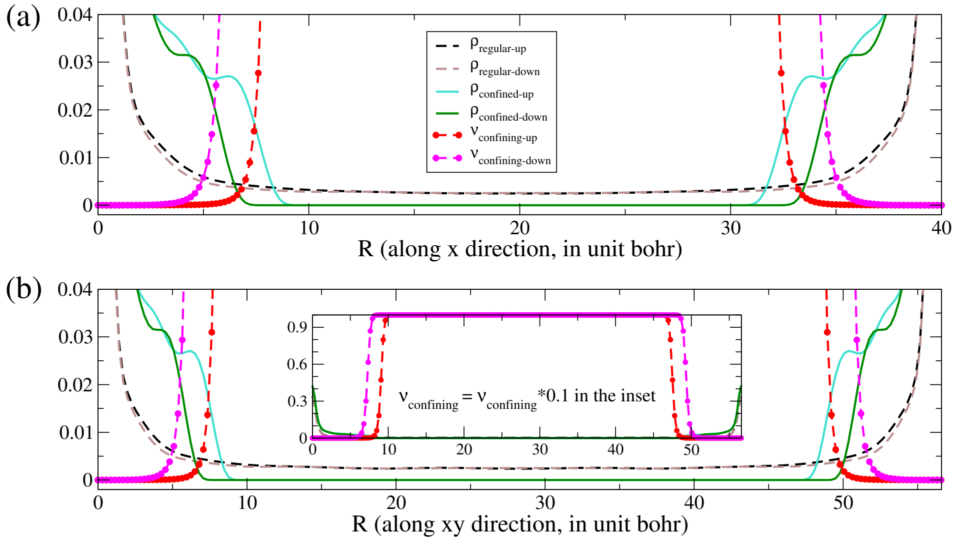


FIG. 11. (color online) The total electron densities $\rho$ (for the lowest 120 orbitals including both occupied and unoccupied orbitals) and confining potential $\nu$ of both spins added along x and xy directions in the xy plane (z=0) for a 24-atom supercell at $R = 0.9\,\mathrm{a_B}$ with k-point (0, 0, 0.075) from DFT non-self-consistent calculations.

Figure 11 shows the total electron densities (for the lowest 120 orbitals including both occupied and unoccupied orbitals) and confining potential added along x and xy directions in the xy plane (z=0) for a 24-atom supercell at $R = 0.9\,\mathrm{a_B}$ with k-point (0, 0, 0.075) from DFT non-self-consistent calculations. The electron densities from regular DFT calculations (without confining potential) are always finite in the xy plane, which indicate that the orbitals are unbounded. Once the confining potential term is added, the electron densities go to zero rapidly and all of the orbitals become bounded.

Expressed in this basis, the effective down-folded Hamiltonian is given by one-body and two-body terms whose matrix elements read

$$h_{pq} = \langle \chi_p | \hat{H}_1 | \chi_q \rangle \ , \ (pr|qs) = \langle \chi_p \chi_q | \hat{H}_2 | \chi_r \chi_s \rangle \ . \tag{17}$$

Here $\hat{H}_1$ includes all one-body terms in the Hamiltonian and $\hat{H}_2$ is the two-body interaction term. These matrix elements, which encode the periodicity and the Coulomb interaction in the underlying supercell, can be efficiently computed using fast Fourier transform techniques, as the orbitals $\chi_p$ are expressed as linear combination of plane waves, and define a Hamiltonian operator that can be treated by any first-principles methodology operating in second quantization. In the present work, we used the

AFQMC to study the down-folded Hamiltonian. For calculations in periodic systems away from the gamma point, the electron repulsion integral has 4-fold symmetry, as opposed to the 8-fold symmetry observed in molecules, which in turn requires to slightly modify the stochastic representation of the imaginary-time evolution in AFQMC calculations [28, 29]. Use of the down-folding techniques allows first-principles (in this case AFQMC) calculations to be performed with a compact Hamiltonian, while retaining material-specific properties.

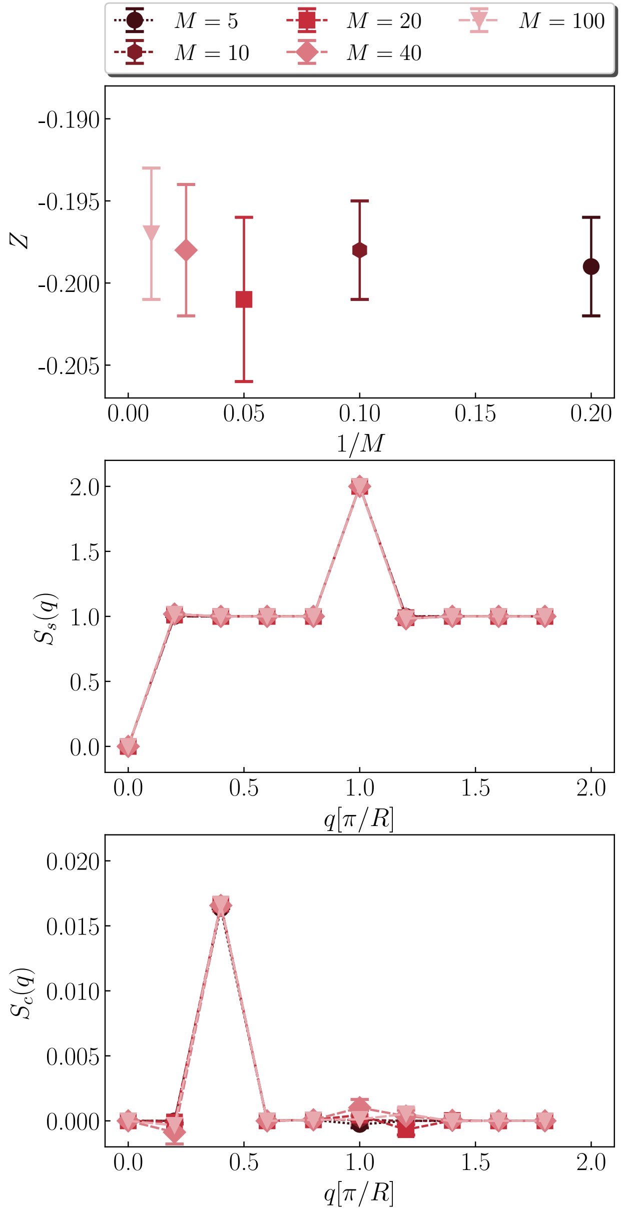


FIG. 12. (color online) Convergence of AFQMC localization measure $Z$ at $R = 3.6\,\mathrm{a_B}$ (top), spin structure factor $S_s(q)$ at $R = 0.9\,\mathrm{a_B}$ (middle) and charge structure factor $S_c(q)$ at $R = 0.9\,\mathrm{a_B}$ (bottom) with basis set size $M$ (dark to light red), using a 2-atom supercell.

In Figure 12 we show the convergence of AFQMC properties for 2-atom supercells at $R = 0.9\,\mathrm{a_B}$ (structure factors) and $R = 3.6\,\mathrm{a_B}$ (localization) with the size $M$ of the KS basis.

### 2. *Additional data*

In Figure 13, we the study the half-filled one-dimensional Hubbard model to check if it can capture the dimer order. Since there is no sign problem, the standard metropolis AFQMC algorithm [30, 31] is used and the force bias technique is applied to

accelerate [32] the Monte Carlo sampling. We set time step $\tau = 0.01$, projection time $\beta = 64t$, and only measure the physical quantities between $20t$ and $44t$.

For the open boundary condition, we measure the nearest neighbor hopping $\hat{h}_i = \sum_\sigma \hat{a}^\dagger_{i+1\sigma}\hat{a}_{i\sigma}$ and find the dimer order along the chain. For the periodic boundary condition, the correlation function $\hat{h}_0\,\hat{h}_i$ is measured, which shows the same behavior. Since there is no long range order at one dimensional systems, we measure the logarithm of the dimerization order versus logarithm of distance and find that the order follows a power-law decay. A free electron wave function is also shown in Figure 13, which basically have the same behavior with a faster decay component.

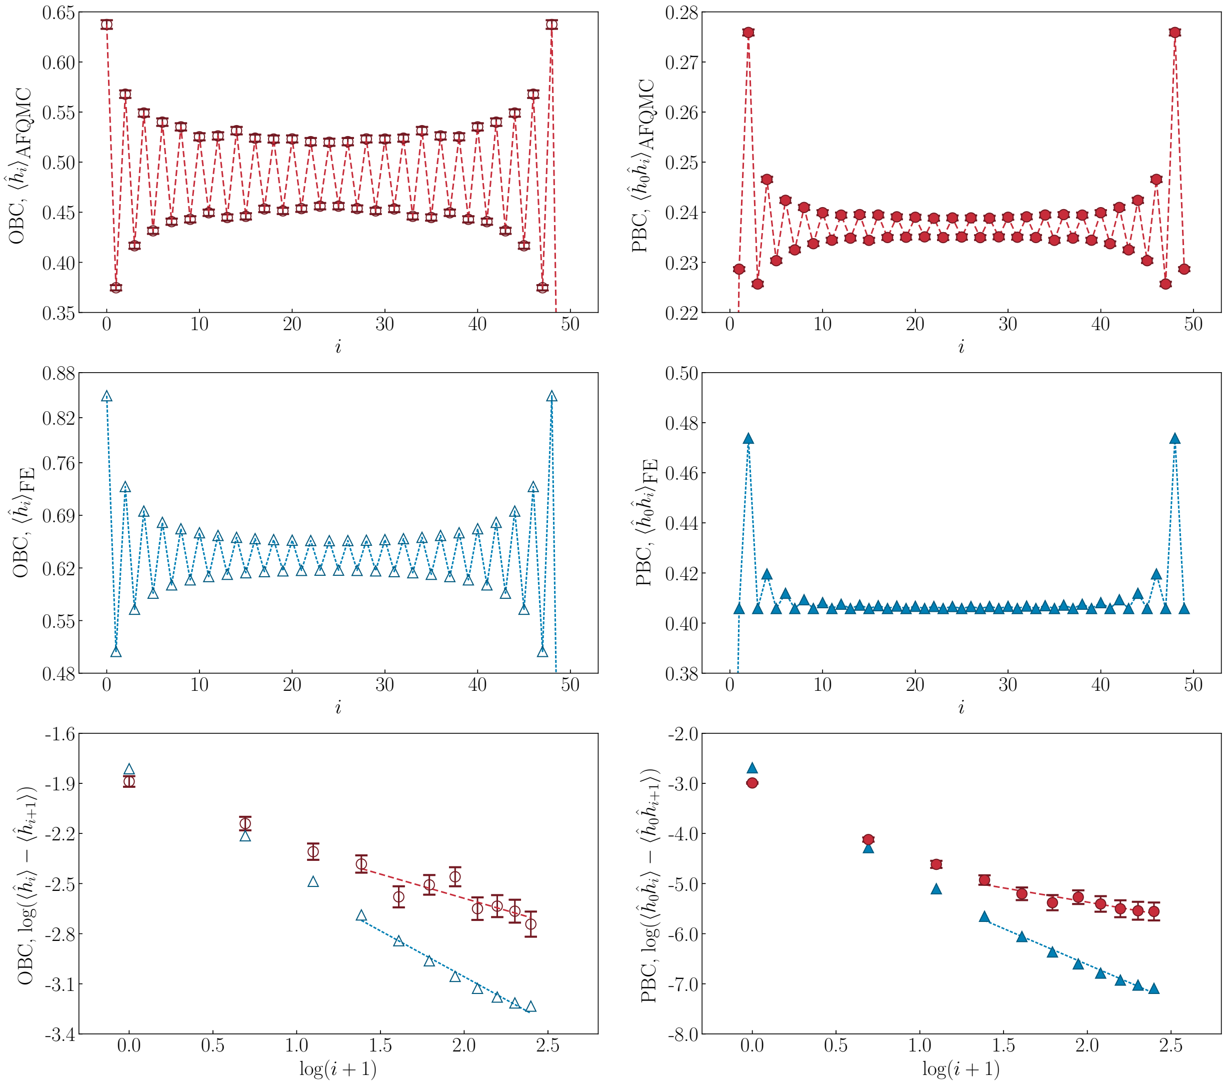


FIG. 13. (color online) Left: expectation value of the hopping operator $\hat{h}_i = \sum_\sigma \hat{a}^\dagger_{i+1\sigma}\hat{a}_{i\sigma}$ for a 50-site Hubbard model with OBC using AFQMC (top, empty red circles) and the free-electron wave-functions (middle, empty blue triangles), and power-law decay in $\langle \hat{h}_i \rangle - \langle \hat{h}_{i+1} \rangle$ (bottom). Right: expectation value of the product $\hat{h}_0\,\hat{h}_i$ for a 50-site Hubbard model with PBC, using AFQMC (top, filled red circles) and the free-electron wavefunction (middle, filled blue triangles), and power-law decay in $\langle \hat{h}_0\,\hat{h}_i \rangle - \langle \hat{h}_0\,\hat{h}_{i+1} \rangle$ (bottom). Results of the fits in the bottom panels are given in Table I.

| method | $\alpha$ (correlation in PBC) | $\alpha'$ (local order in OBC) |
|---|---|---|
| FE | 1.44(7) | 0.55(3) |
| AFQMC | 0.57(8) | 0.29(7) |

TABLE I. Power-law decay in $\langle \hat{h}_i \rangle - \langle \hat{h}_{i+1} \rangle$ for a 50-site Hubbard model with OBC, and in $\langle \hat{h}_i \hat{h}_0 \rangle - \langle \hat{h}_{i+1} \hat{h}_0 \rangle$ for a 50-site Hubbard model with PBC. In both cases, the quantity of interest is fit to the functional form $\propto 1/(i+1)^{\alpha}$.

### C. Coupled cluster (CC)

Ground-state coupled cluster (CC) calculations assume an ansatz of the form

$$|\Psi\rangle = e^{\hat{T}}|\Phi\rangle \tag{18}$$

where $\hat{T}$ is a sum over particle-hole type excitations and $|\Phi\rangle$ is a reference determinant, here chosen as a Hartree-Fock determinant. In this work, we use coupled cluster singles and doubles (CCSD), where $\hat{T}$ is limited to 1 particle-1 hole (1p1h) and 2 particle-2 hole (2p2h) excitations. Gaps are calculated using equation-of-motion coupled cluster (IP/EA-EOM-CC). In this case, the $N-1$ and $N+1$ wavefunctions are written in the form

$$|\Psi^{\pm}\rangle = \hat{R}^{\pm}e^{\hat{T}}|\Phi\rangle \tag{19}$$

where $\hat{R}^{+}$ generates the electron attached state, and $\hat{R}^{-}$ the electron ionized state. At the approximation level in this work (EA-EOM-CCSD, IP-EOM-CCSD) $\hat{R}^{+}$ generates 1p, 2p1h excitations, and $\hat{R}^{-}$ generates 1h, 2h1p excitations.

#### 1. *Computational details*

Hartree-Fock reference calculations were carried out on H atom circular rings of varying length (from 70 to $> 500$). In the limit of infinite H atoms, this will give the same thermodynamic limit as the periodic boundary condition calculations. We used several different basis sets including uncontracted STO-3G, STO-6G, aug-cc-pVDZ, and an even-tempered basis supplemented with mid-bond basis functions (the uncontraction was used to provide the flexibility to capture both valence like states and diffuse states associated with the second band). We found that the qualitative nature of the results presented below were consistent between the above bases, and that the character of the second band ($2s$ vs $2p$) did not significantly modify the resulting picture. For each bond length, we attempted to converge a wide range of Hartree-Fock solutions corresponding to different kinds of symmetry breaking, as well as different fillings of the upper and lower bands (see below). Ground-state and equation of motion coupled cluster calculations were then carried out starting from the different Hartree-Fock solutions for rings of up to length 110. EOM-CC gaps were extrapolated to the thermodynamic limit using a simple $1/L$ formula.

#### 2. *Hartree-Fock reference state*

The coupled cluster calculations require a choice of the initial state $|\Phi\rangle$. As traditionally done in coupled cluster calculations, we used Hartree-Fock reference states. It is possible to find multiple kinds of Hartree-Fock solutions. We classify the orbitals as symmetry adapted (sa) ($N_{\uparrow} = N_{\downarrow}$ in a band) when the orbitals preserve the translational symmetry of the lattice and are identical for up and down spin; broken symmetry (bs) orbitals ($N_{\uparrow} = N_{\downarrow}$ in a band), which are accompanied by antiferromagnetic order; or ferromagnetic orbitals (fm) ($N_{\downarrow} = 0$ in a band). At shorter bond lengths where two bands are occupied, it is possible to find stable Hartree-Fock solutions for different choices of partitioning of the electrons between the upper and lower bands. The variety of Hartree-Fock solutions that can be found creates significant complexity.

In Fig. 14 we show on the right side the energy lowering due to the occupation of the second band compared to the state with a single band occupied. On the left side we show the corresponding fractional filling of the second band. In these calculations we only used sa orbitals. Note that at intermediate to short bond-lengths a ferromagnetic character in the upper band is lower in energy, while at very short bond lengths a paramagnetic solution with no magnetic character in either band is preferred. The smooth evolution of the upper band filling is indicative of metallic character.

Fig. 15 is a representative plot of the HF energy with a sa character at each bond length with different numbers of electrons in the upper band (reasonably well converged to the basis set and thermodynamic limits). One sees the optimal 2nd band filling as the dark band of results; other fillings may be then be regarded as reflecting netural excitations. It is clear from this plot that the energy evolves relatively smoothly with filling. Moreover, at any given $R$, there are multiple solutions (with varying upper band filling) within a small energy window, as indicated by the wide band formed around the optimal filling white line.

Fig. 16 shows the HOMO-LUMO gap at a highly compressed bond-length for different characters of HF solutions, as a function of the number of atoms $N$ in the simulated ring. One sees that, out of the different types of Hartree-Fock solution, with different kinds of order, one can find both insulating ones (where the gap does not vanish in the thermodynamic limit) and metallic ones (with vanishing gap). We regard the solutions with insulating character at compressed bond lengths as artifacts of mean-field symmetry-broken states which typically open a gap to develop long-range order.

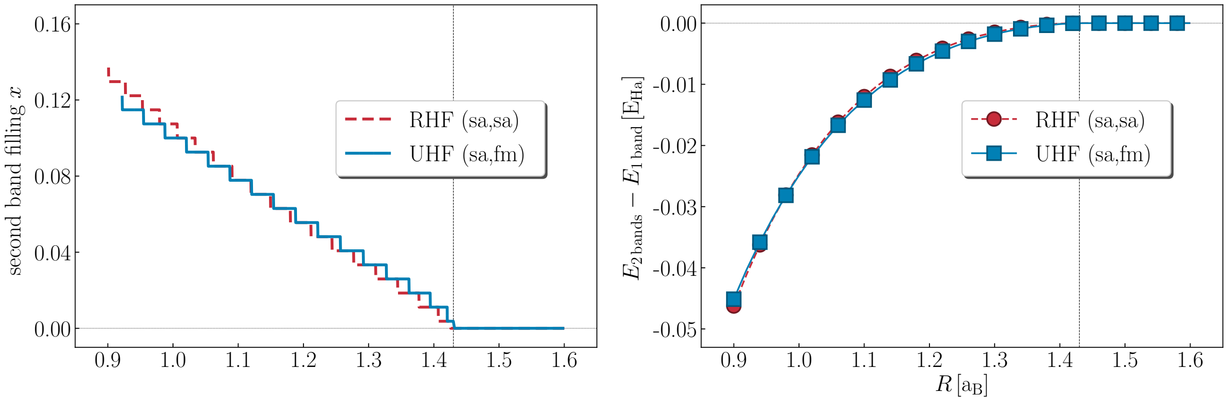


FIG. 14. (color online) Hartree-Fock filling of the second band for short $R$ (left) and corresponding lowering of the energy (right), allowing for sa (red circles) or fm (blue squares) character in the second band.

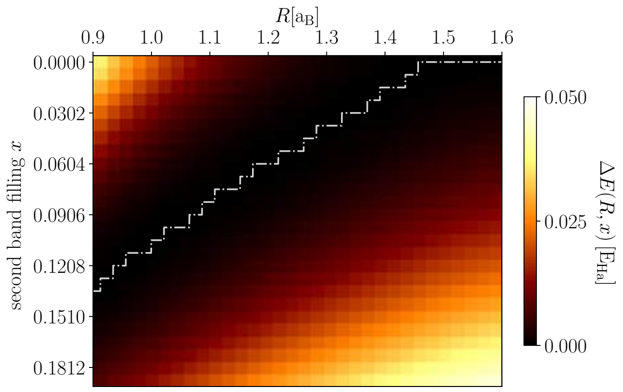


FIG. 15. (color online) Hartree-Fock energy as a function of $R$ and filling of the second band $x$.

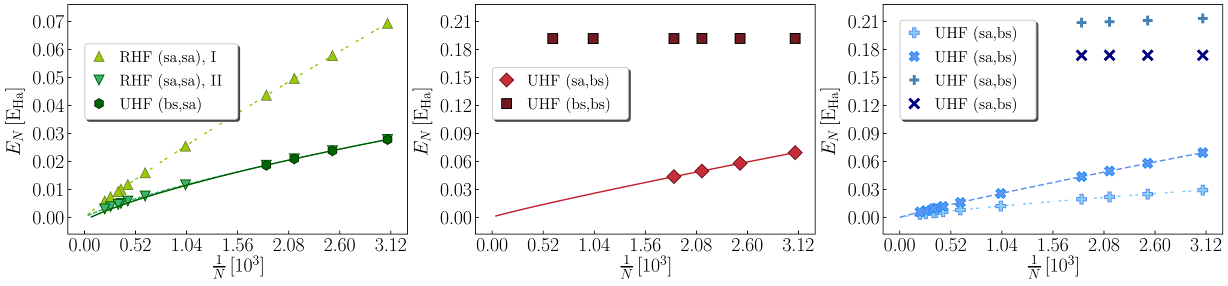


FIG. 16. (color online) Hartree-Fock HOMO-LUMO gap for $R = 0.96\,\mathrm{a_B}$, uncontracted STO-3G basis, with sa (symmetry adapted, $N_\uparrow = N_\downarrow$), bs (broken symmetry, $N_\uparrow = N_\downarrow$) or fm (ferromagnetic, $N_\downarrow = 0$) character in each band.

### 3. *Coupled cluster solutions*

Starting from the Hartree-Fock solutions, one can then compute the coupled cluster wavefunctions and gaps. Although the coupled cluster ground state depends on the nature of the HF reference used, we have chosen to work with metallic HF solutions at very short bond lengths.

In Fig. 17 we show the EOM-CC charge gaps extrapolated to the TDL computed from representative CC solutions. The extrapolated EOM-CCSD gaps vanish at short bond-lengths, indicating metallic character. The large magnitude of the EOM-CCSD gaps observed in the insulating regime can be attributed to the incomplete basis set used. The fact that both CCSD and UCCSD predict insulating character at long bond lengths can be regarded as a consistency check. Based on these calculations, the metal-insulator transition is predicted to take place between $R = 1.1$ and $R = 1.6$ a.u., in agreement with other measures in this work.

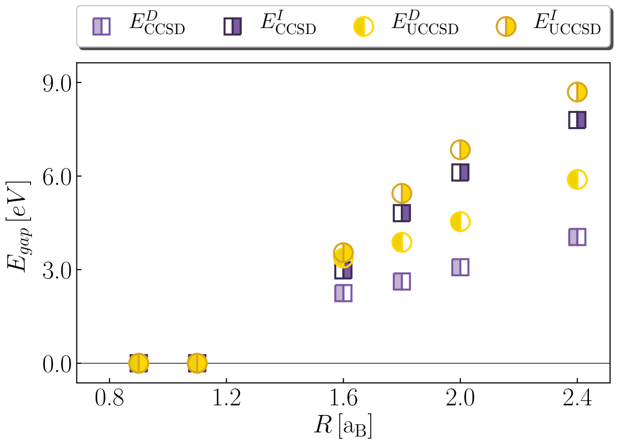


FIG. 17. (color online) EOM-CCSD (violet squares) and EOM-UCCSD (yellow circles), charge gaps. Direct (left-filled symbols) and indirect (right-filled symbols) gaps are shown.

### D. Density-matrix renormalization group

#### 1. Gaussian basis convergence

To obtain a compact basis with which to carry out DMRG calculations, we started with a standard augmented correlation-consistent Gaussian basis [33] with periodic boundary conditions (PBC) and different twist $\mathbf{k}$ values (here $\mathbf{k} = 0.0, 0.1, \cdots, 0.5$). The basis of the system is then a set of $\mathbf{k}$-adapted Gaussian basis functions [34, 35],

$$\phi_\mu^{\mathbf{k}}(\mathbf{r}) = \sum_{\mathbf{T}} \mathrm{e}^{\mathrm{i}\mathbf{k}\cdot\mathbf{T}} \phi_\mu^{\mathbf{T}}(\mathbf{r} - \mathbf{T}) \tag{20}$$

where the summation over lattice vector $\mathbf{T}$ is converged with respect to repeated cell images.

To assess the rate of convergence of such a crystalline basis for the hydrogen chain we carried out Hartree-Fock, 2$^{\mathrm{nd}}$ order Moller-Plesset (MP2), CCSD, and full configuration interaction (FCI) calculations (where possible) for a $H_2$ unit cell with PBC and $H_{10}$ molecule with OBC in the aug-cc-pVDZ, aug-cc-pVTZ, and aug-cc-pVQZ bases (aug-DZ, aug-TZ, aug-QZ), as well as the non-augmented bases cc-pVDZ, cc-pVTZ, cc-pVQZ, cc-pV5Z (DZ, TZ, QZ, 5Z). Selected results for the $H_2$ cell are in Table II, and for the $H_{10}$ molecule in Table III.

TABLE II. Hartree-Fock energy, MP2 and FCI correlation energies (per atom) in Hartrees, $H_2$ unit cell at PBC ($R = 0.9\,\mathrm{a}_B$). $N_{\mathrm{AO}}$ denotes number of atomic orbitals (for $H_2$'s).

| | $N_{\mathrm{AO}}$ | HF | MP2 | FCI |
|---|---|---|---|---|
| aug-DZ | 18 | -1.63622 | -0.01167 | -0.02401 |
| aug-TZ | 46 | -1.68709 | -0.01432 | -0.02588 |
| aug-QZ | 92 | -1.68826 | -0.01576 | -0.02721 |
| 5Z | 110 | -1.68844 | -0.01620 | -0.02753 |

TABLE III. Hartree-Fock energy, MP2 and CCSD correlation energies (per atom) in Hartrees, $H_{10}$ molecule at OBC ($R = 1.0\,\mathrm{a}_B$). CBS estimate from extrapolated sliced basis calculation [36]. $N_{\mathrm{AO}}$ denotes number of atomic orbitals (for $H_{10}$'s).

| | $N_{\mathrm{AO}}$ | HF | MP2 | CCSD |
|---|---|---|---|---|
| DZ | 50 | -0.40101 | -0.01740 | -0.02046 |
| TZ | 140 | -0.41393 | -0.02227 | |
| QZ | 300 | -0.41505 | -0.02337 | |
| 5Z | 550 | -0.41550 | -0.02377 | |
| aug-QZ | 90 | -0.40721 | -0.01887 | -0.02185 |
| aug-TZ | 230 | -0.41495 | -0.02257 | -0.02517 |
| aug-QZ | 460 | -0.41566 | -0.02352 | |
| CBS | | -0.41575 | | |

From these tables, we observe systematic convergence of both the Hartree-Fock and FCI energy as the basis size is increased, however, the FCI energy converges much more slowly due to the need to capture the electron-electron cusp. We also see that augmented bases perform better than non-augmented bases due to the need to capture diffuse upper bands in the metallic (short $R$) regime of the H chain. As a compromise between cost and accuracy, we chose to use the aug-TZ basis as the basis for subsequent calculations, because *both* the mean-field and correlation energy are converged to within about 1mH per atom in this basis.

#### 2. Natural orbital basis for DMRG calculations

To further compress the basis for the DMRG calculations, we constructed natural orbitals from the MP2 wavefunction. We then truncated the Hilbert space to a dimension of $N_{\mathrm{b}}$ natural orbitals per hydrogen atom. Such a Hilbert space is referred to as a complete active space (CAS) in this procedure. An analogous truncation of the mean-field orbitals is referred to as downfolding

in the AFQMC context. The convergence of the natural orbital and Hartree-Fock (downfolded) active spaces for the correlation energy can be seen in test MP2 calculations on a $H_{10}$ system. Here the underlying aug-cc-pVTZ basis is projected onto the MP2 natural orbital CAS and downfolded Hartree-Fock CAS with different values of $N_\mathrm{b}$ (for test purposes, we used open boundary conditions). The percentage of MP2 correlation energy recovered by the active space is shown in Fig. 18. Note that by using

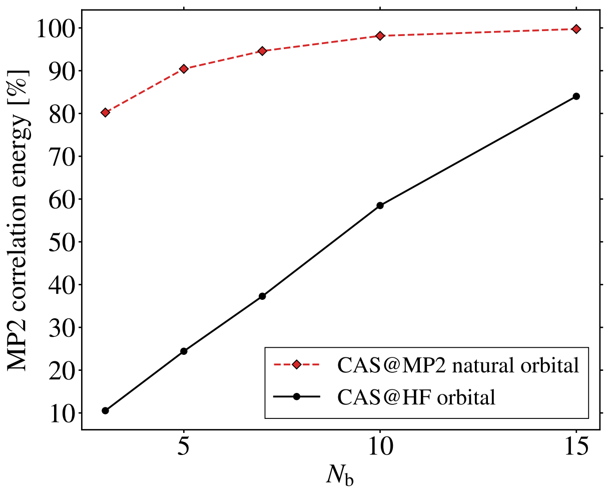


FIG. 18. The MP2 correlation energy captured by different numbers of bands $N_\mathrm{b}$ with Hartree-Fock orbitals or MP2 natural orbitals.

natural orbitals, with $N_\mathrm{b} = 5$ one already captures about 90 % of the correlation energy in this system. In the following DMRG calculations, we keep $N_\mathrm{b}$ fixed at 5.

### 3. *DMRG wavefunction and computational protocol*

The density matrix renormalization group (DMRG) [37] uses a matrix product state (MPS) as the wavefunction ansatz,

$$|\Psi\rangle = \sum_{n_1, n_2, \cdots, n_L} \mathbf{A}^{n_1} \mathbf{A}^{n_2} \cdots \mathbf{A}^{n_L} |n_1 n_2 \cdots n_L\rangle \tag{21}$$

where $L$ is the number of orbitals in the system and the wavefunction amplitudes are decomposed into a product of tensors $\mathbf{A}^n$. The tensors $\mathbf{A}^n$ (other than $\mathbf{A}^{n_1}$ and $\mathbf{A}^{n_L}$) are matrices of dimension $D \times D$ for a given $n$; $D$ is termed the bond dimension, and controls the accuracy of the DMRG algorithm. As $D$ approaches infinity, DMRG becomes exact. For the ground-state of a quasi 1D system, such as the hydrogen chain, $D$ can be truncated to a relatively small number independent of the chain length, while keeping a constant accuracy (per atom). The coefficients of $\mathbf{A}^n$ are then variationally optimized by the DMRG sweep algorithm [38] so that the energy of the system is minimized. The standard way to apply DMRG in a chemical system is to express the Hamiltonian in a finite orthogonal orbital basis [39]. Consequently, the Hamiltonian that is used is that in Eq. 5. For all calculations we used (split-localized) MP2 natural orbitals [(L)MO] derived from a large Gaussian basis (see above Section II D 1) except for the single plot in Fig. 1 which was carried out in a minimal (STO-6G) basis.

To perform the DMRG calculations, we followed the strategy described in Ref. [40]. Aside from the minimal basis calculation carried out for $H_{50}$ in the manner described in Ref. [3], split localization of the natural orbitals was carried out with the Edmiston-Ruedenberg (ER) method [41] for the natural orbitals of occupied and virtual character. The local orbitals were then reordered by the Fiedler algorithm [40]. We carried out a spin-adapted DMRG algorithm, as implemented in the BLOCK program [42–45], for a $H_{24}$ chain with various twists at $R = 0.9\,\mathrm{a}_B$ and $R = 2.5\,\mathrm{a}_B$. The maximum bond dimension $D$ was limited to 1000 and the ground state energy was converged to better than 0.01 mH per atom. The one- and two-particle reduced density matrices were then computed both for the natural orbital analysis and to compute the spin structure factor $S(q)$ [see Sec. II B for the formula for $S(q)$].

### 4. *Additional data*

*a.* $\mathbf{k}$*-resolved spin structure factor* We show the spin structure factor $S(q)$ at different twists $\mathbf{k}$ in Fig. II D 4 a. At $R = 0.9\,\mathrm{a}_B$, the $S(q)$ at the $\Gamma$ point shows a different peak position (i.e. $q_2$ in the main text), compared to $S(q)$ at other twists $\mathbf{k}$s.

This qualitative difference indicates the difference of orbital character with this boundary condition (see below for more details). At $R = 2.5\,\mathrm{a}_B$, although the peak values for different twists $\mathbf{k}$s are different, the peak positions are the same.

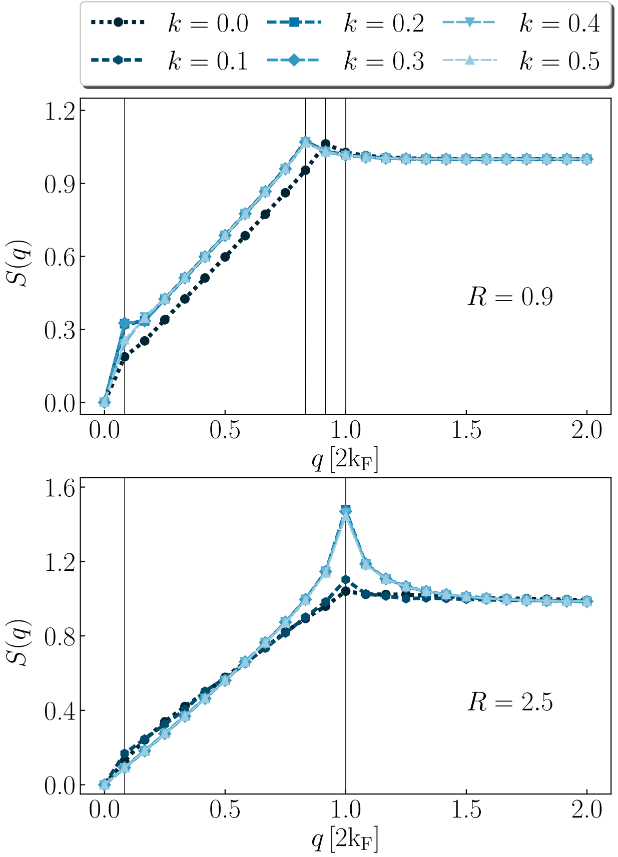


FIG. 19. Spin structure factor as a function of $q$, $k$ from DMRG, at $R = 0.9\,\mathrm{a}_B$ (top) and $R = 2.5\,\mathrm{a}_B$ (bottom).

*b. Orbital character analysis on DMRG natural orbitals* We project the DMRG natural orbitals onto the crystalline Gaussian atomic orbital basis used in the mean-field calculation in order to analyze their character. Note that in the atomic orbital basis, the $s$, $p_z$ and $d_{z^2}$ orbitals are of the same symmetry along the bonding direction and are thus $\sigma$-like orbitals. $p_x$ and $d_{xz}$ ($p_y$ and $d_{yz}$) are of the same symmetry orthogonal to the bonding direction and should be classified as $\pi$-like orbitals. As shown in the main text, at $R = 0.9\,\mathrm{a}_B$, establishing the orbital character around Fermi level is a delicate problem influenced by the computational method and boundary conditions such as the $\mathbf{k}$ twist. In Fig. 20, we collect the orbital characters of the first 20 natural orbitals of $H_{24}$ at $R = 0.9\,\mathrm{a}_B$ from DMRG at three representative $\mathbf{k}$ values (0.0, 0.1 and 0.5). At the $\Gamma$ point, the orbitals around the Fermi level are $\sigma$-like ($s$-like). However, at $\mathbf{k} = 0.1$ and $\mathbf{k} = 0.5$, the frontier orbitals contain a mix of $s$ and $p$ character. The change in orbital character also influences the occupancy and spin structure factor. In contrast, at $R = 2.5\,\mathrm{a}_B$, all orbitals are $s$-like (see Fig. 21).

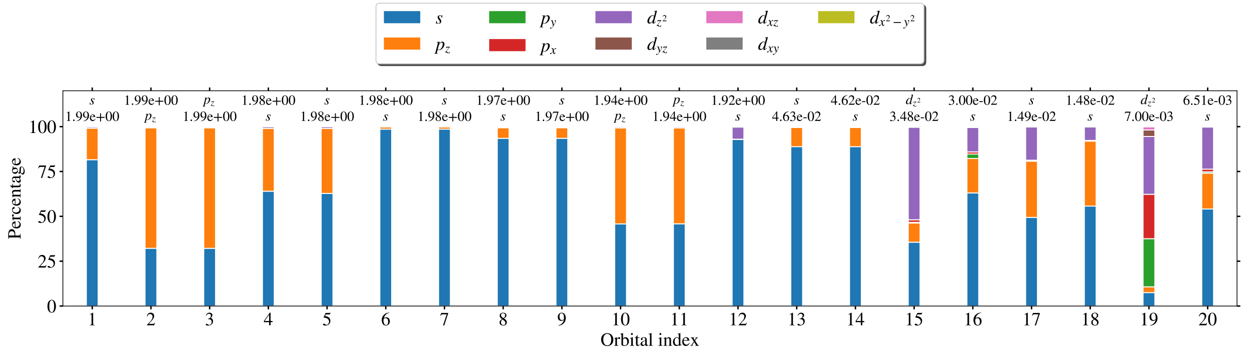


(a)$\mathbf{k} = 0.0$

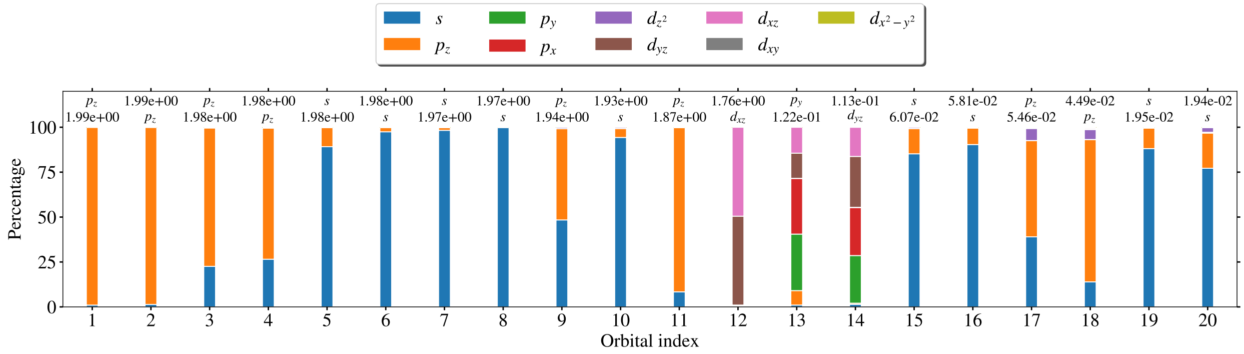


(b)$\mathbf{k} = 0.1$

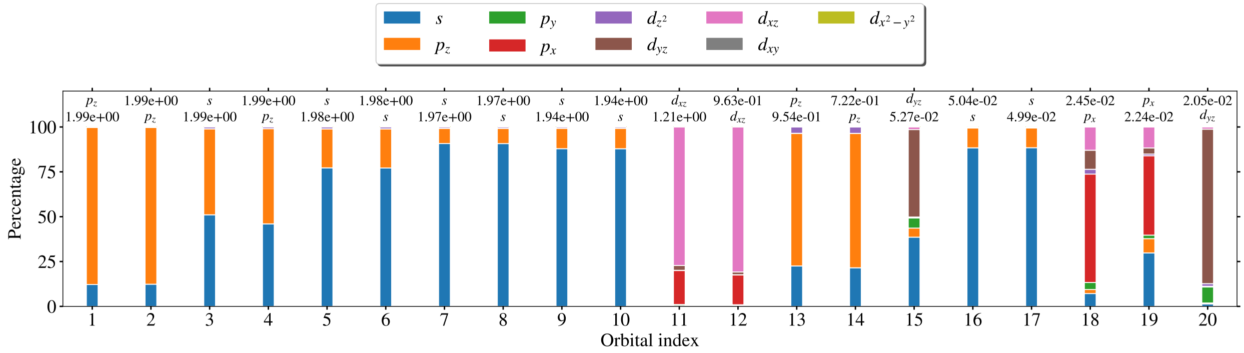


(c)$\mathbf{k} = 0.5$

FIG. 20. Orbital character and natural occupancy of the first 20 DMRG natural orbitals of $H_{24}$ at $R = 0.9\,\mathrm{a}_B$.

### E. Sliced-basis density-matrix renormalization group (sb-DMRG)

#### *1. Approach*

Sliced-basis DMRG (sb-DMRG)[46] runs standard DMRG within a specialized basis set that uses a real-space grid along one direction and defines localized basis functions, spanning the transverse direction, at each grid point(defining a ”slice”). The merits of using such a basis set manifest as a reduction in the number of interaction terms, going from the usual quartic scaling to only quadratic in the number of grid points while also maintaining area-law entanglement scaling. In addition to these advantages, an SVD compression of the long-range interactions produces an MPO with a modest bond dimension which is nearly independent of the size of the system. This technique allows the method to scale essentially linearly with the number

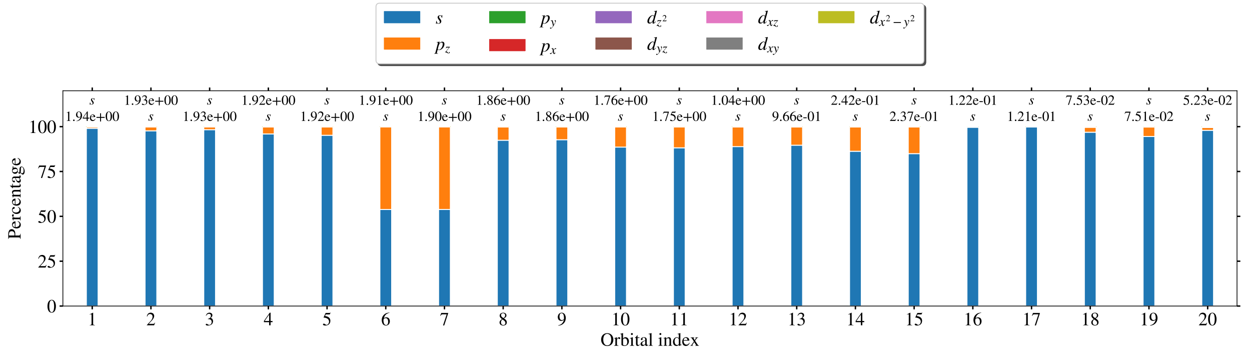


(a)$\mathbf{k} = 0.0$

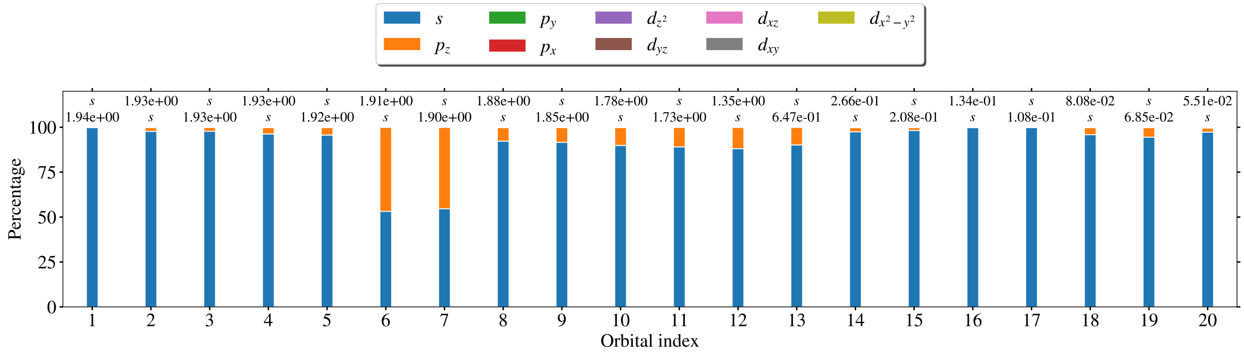


(b)$\mathbf{k} = 0.1$

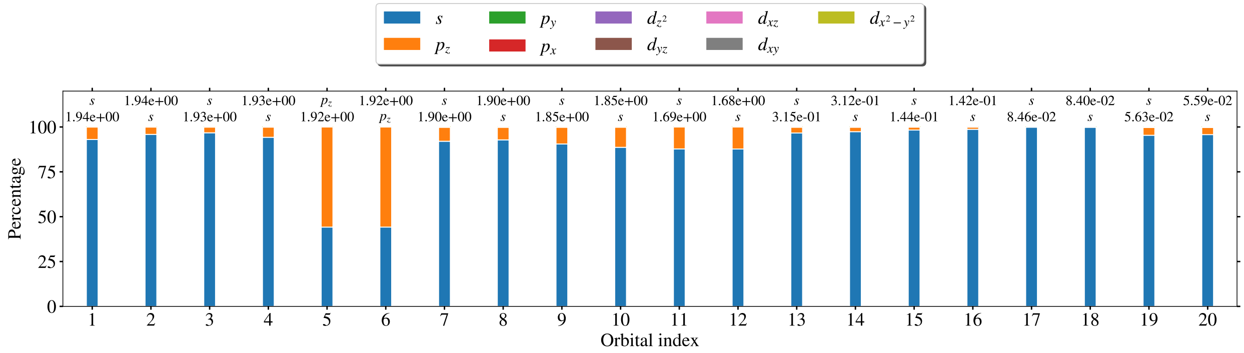


(c)$\mathbf{k} = 0.5$

FIG. 21. Orbital character and natural occupancy of the first 20 DMRG natural orbitals of $H_{24}$ at $R = 2.5\,\mathrm{a}_B$.

of atoms.

*a. Sliced-basis Hamiltonian* Starting from the usual electronic structure Hamiltonian for fixed nuclei,

$$\hat{H} = \int_{\mathbf{r}} \hat{\psi}^\dagger_\sigma(\mathbf{r}) \left[ -\frac{1}{2}\nabla^2 + v(\mathbf{r}) \right] \hat{\psi}_\sigma(\mathbf{r}) + \frac{1}{2}\int_{\mathbf{r},\mathbf{r}'} \frac{1}{|\mathbf{r}-\mathbf{r}'|} \hat{\psi}^\dagger_\sigma(\mathbf{r})\hat{\psi}^\dagger_{\sigma'}(\mathbf{r}')\hat{\psi}_{\sigma'}(\mathbf{r}')\hat{\psi}_\sigma(\mathbf{r}) \tag{22}$$

the sliced basis functions are constructed by defining a real-space grid along the $\hat{z}$ direction with grid spacing, $a$, and local basis functions $\{\phi_i(x, y)\}$, $j = 1, 2, ..., N_o$ restricted to live on each point, $n = 1, 2, ..., N_z$. Within this basis, the Hamiltonian in (22)

may be written as,

$$\hat{H} = \frac{1}{2}\sum_{nn'}\sum_{ij} t_{ij}^{nn'} \hat{c}_{\sigma ni}^{\dagger}\hat{c}_{\sigma n'j} + \frac{1}{2}\sum_{nn'}\sum_{ijkl} V_{ijkl}^{nn'} \hat{c}_{\sigma ni}^{\dagger}\hat{c}_{\sigma' n'j}^{\dagger}\hat{c}_{\sigma' n'k}\hat{c}_{\sigma nl} \quad (23)$$

where, for $\boldsymbol{\rho} = (x, y)$,

$$t_{ij}^{nn'} = \delta_{nn'} \int_{\boldsymbol{\rho}} \phi_i(\boldsymbol{\rho}) \left[ -\frac{1}{2}\nabla_{\boldsymbol{\rho}}^2 + v(\boldsymbol{\rho}, z_n) \right] \phi_j(\boldsymbol{\rho}) - \delta_{ij}\frac{1}{2a^2}\Delta_{nn'} \quad (24)$$

$$V_{ijkl}^{nn'} = \int_{\boldsymbol{\rho},\boldsymbol{\rho}'} \frac{\phi_i(\boldsymbol{\rho})\phi_j(\boldsymbol{\rho}')\phi_k(\boldsymbol{\rho}')\phi_l(\boldsymbol{\rho})}{\sqrt{|\boldsymbol{\rho} - \boldsymbol{\rho}'|^2 + (z_n - z_{n'})^2}} \quad (25)$$

The first term in (24) represents the intra-slice hopping and one-body potential terms whereas the second term represents the inter-slice hopping where the matrix $\Delta_{nn'}$ comes from approximating the derivatives in the $\hat{z}$ direction with finite differences. For the interactions in (25), the restriction that each local transverse function must live on a slice reduces the total number of terms from $N_z^4 N_o^4$ to just $N_z^2 N_o^4$.

In a typical sb-DMRG calculation, both the $1/r$ decay and functions $\{\phi_i(x, y)\}$ in (25) can be expressed in terms of Gaussians, the former by a fitting procedure and the latter by using standard Gaussian basis sets(see next section). So in addition to reducing the number of terms, the integrals become trivial Gaussian integrals which may be stored in tables, making the calculation of these integrals very fast.

*b. Constructing the Transverse Functions* The transverse functions are constructed from standard Gaussian basis set functions which are defined by three numbers, $(\zeta, n, m)$ with each function taking the form,

$$g(x, y) = \sqrt{\frac{2\zeta}{\pi}} x^n y^m e^{-\zeta(x^2+y^2)} \quad (26)$$

The values of $n$ and $m$ determine the character of the function(i.e. $s$-type, $p$-type etc.) and $\zeta$ controls the width. In some basis sets, these primitive Gaussians are contracted with others of the same type to form new basis functions. sb-DMRG goes one step further and uses the $N$ contracted Gaussians to form $N_o \leq N$ functions, $\{\phi_i(x, y)\}$. Unlike the contracted Gaussians, these functions are orthonormal allowing the integrals used to calculated the Hamiltonian parameters to take a simpler form.

First, an uncontracted orthonormal basis is formed from the $N_g$ primitive Gaussians by orthogonalizing each function to the rest. The $N$ contracted Gaussians are then projected into this basis, giving a vector $\boldsymbol{\eta}_j$ for the $j^{th}$ contracted Gaussian. A density matrix is then formed from the outer product of these vectors and subsequently diagonalized. The first $N_o$ eigenvectors are taken to be an optimal representation of the space spanned by the full contracted Gaussians and are projected back into the original uncontracted orthonormal basis. This defines a mapping between the ”optimal” representation and the primitive Gaussians which may be used to calculate the Hamiltonian parameters of the previous section.

In the main text, the sb-DMRG calculations are done using the basis shown in Fig. 22. This basis set is a slight modification of the one defined in the appendix of [3] which is just cc-pVDZ augmented with two diffuse orbitals at $\zeta = 0.2$ and $\zeta = 0.05$.

### 2. *Boundary Conditions at small Atomic Spacing*

For H-Chain systems with atomic spacing $R > 1.4a_B$, regions of about $10a_B$ on either side of the first and last atom are included in the discretization to better control for finite-size effects within sb-DMRG. However, for $R \leq 1.4a_B$, electrons that have been pushed out of the main $1s$ band may begin to occupy these edge regions.

A useful quantity to study this is what we are calling the spread, namely $\langle x^2 + y^2 \rangle$ versus $z$. Specifically, given the single particle electron density $\rho(x, y, z)$, the spread is

$$\langle r^2 \rangle (z) = \frac{\int dxdy\ (x^2 + y^2)\rho(x, y, z)}{\int dxdy\ \rho(x, y, z)} \quad (27)$$

where $\rho$ is the diagonal part of the Green's function, $G(x, y, z, x', y', z') = \sum_{ij} C_{ij}\phi_i(x, y, z)\phi_j(x', y', z')$, in which the $\phi_j$ are the basis functions and $C_{ij}$ is the Green's function in terms of basis functions. This is essentially a weighted average of the spread of each orbital on a slice in which the weight is determined by the occupancy of the orbitals. Large values of $\langle r^2 \rangle$ indicate either a high occupancy of the more extended orbitals (what we are interested in) or that the ”1s” orbital itself has spread out.

As shown in Fig. 23a, a measure of $\langle r^2 \rangle$ shows a large spread in the edge regions. While this is a legitimate feature of a finite hydrogen chain, it results in a slower convergence to the thermodynamic limit, for which there are no edges. In an infinite

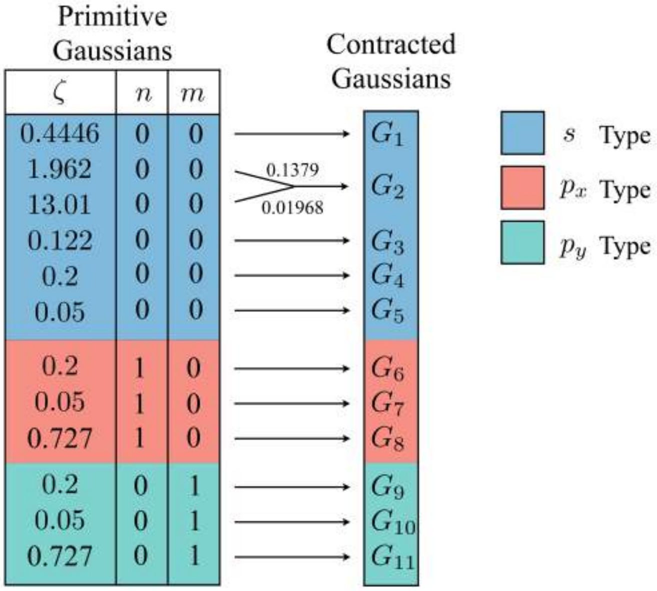


FIG. 22. $N_g = 12$ primitive Gaussians are contracted down to $N = 11$ Gaussians. These Gaussians are then used to construct the transverse functions used in sb-DMRG as described in II E 1 b. There are both wide and narrow Gaussians defined for each type, making the basis set a good representation of the complete basis set limit.

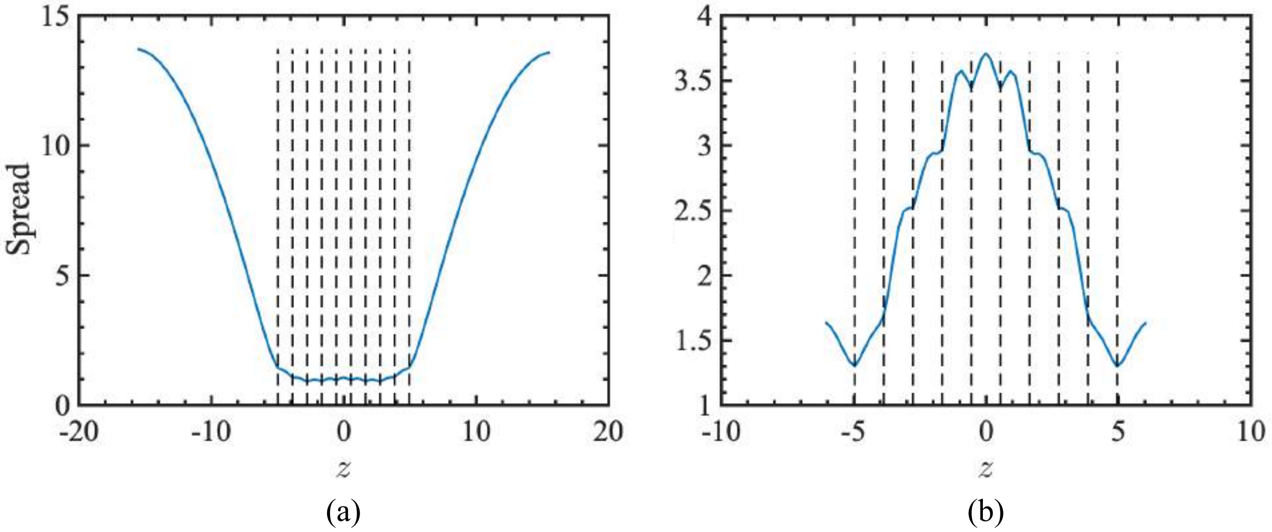


FIG. 23. $\langle r^2 \rangle$ along the chain for H10 at $R = 1.1 a_B$ using the basis defined in [3] (a) before and (b) after truncating the edge regions. The dashed lines indicate the nuclear position.

chain, electrons pushed out of the $1s$ band can only occupy bulk diffuse $2s$ or $2p$ bands. Periodic BCs fix this but are bad for DMRG. Instead, hard walls are placed at a distance $R/2$ beyond the first and last atoms, only in the $z$ direction in order to force the occupancy of the higher bands and keep the electrons within the bulk. Fig. 23b shows the spread after such a truncation for the same system. The occupancy of the bands may then be verified by calculating the slice natural orbital occupancy in which we diagonalize any of the $s$, $p_x$ or $p_y$ blocks of the Green's function confined to a slice. This is plotted in Fig. 24a for the $s$ block of the untruncated chain and in Fig. 24b for the $s$, $p_x$ or $p_y$ blocks of the truncated chain. Beyond the last atom on either edge, the "1s" tends to spread towards the ends before truncation with no occupancy in the $p$ bands. It is only after truncation that the higher orbitals become occupied, which is consistent with the measurement of the spread. This scheme is employed in all sb-DMRG calculations within the main text, mainly to assess the occupancy of the $2s$ and $2p$ as a function of $R$.

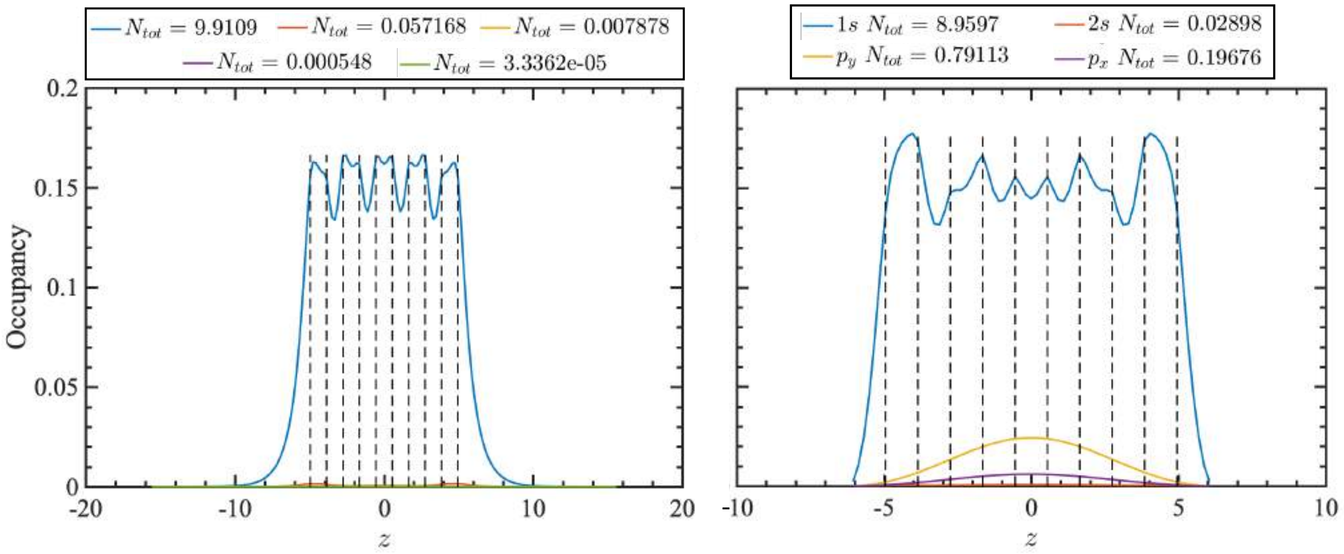


(a) (b)

FIG. 24. (a) $s$ band occupancy per slice for H10 at $R = 1.1a_B$ using the basis defined in [3] without truncating the edge regions. (b) $1s$, $2s$, $p_x$ and $p_y$ occupancy per slice for H10 at $R = 1.1a_B$ using the same basis with truncated edge regions. In both figures, the legend gives the total values of the occupancy after summing over the slices and the dashed lines indicate the nuclear position.

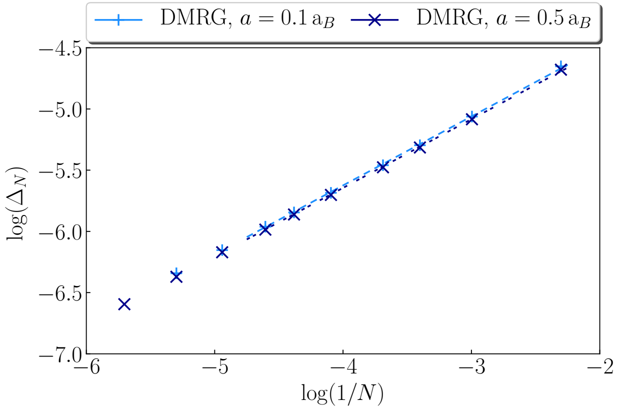


FIG. 25. Dimerization measure $\Delta_N$ as a function of chain size $N$ from sliced-basis DMRG, at $R = 2.0\,\mathrm{a}_B$, using $a = 0.1, 0.5\,\mathrm{a}_B$.

| method | $R\,[\mathrm{a}_B]$ | $d$ |
|---|---|---|
| sb-DMRG, $a = 0.1\,\mathrm{a}_B$ | 2.0 | 0.563(4) |
| sb-DMRG, $a = 0.5\,\mathrm{a}_B$ | 2.0 | 0.552(2) |

TABLE IV. Power-law decay $\Delta_N = \Delta_0\, N^{-d}$ in the dimerization measure, from sliced-basis DMRG.

| basis | $Z_{1s}$ | $Z_{2s}$ | $Z_{3s}$ | $Z_{4s}$ | $Z_{1p}$ | $Z_{2p}$ | $Z_{1d}$ |
|---|---|---|---|---|---|---|---|
| modified-ccpVTZ | 5.095 | 1.159 | 0.3258 | 0.1027 | 1.407 | 0.388 | 1.057 |
| modified-ccpVDZ | 1.962 | 0.4446 | 0.122 | = | 0.2 | 0.05 | = |
| 2-4 body Jastrow | 0.01701 | 0.01701* | 0.5366 | = | 0.3022 | 0.1101 | 0.2656 |

TABLE V. The exponents of the uncontracted gaussian basis sets used in this work both for DFT and QMC calculations. In the small $R \leq 1.4$ region we have obviously adopted only the modified ccpVDZ one (see Fig. 26). The last raw refers to the uncontracted basis used for the so called two (electron-electon) -three (electron-electron-ion) and four body (electron-electron-ion-ion) Jastrow factors that has been optimized for the sample case of ten atoms at $R = 1$. The $Z_{2s}$ exponent marked by $^*$ refers to a standard gaussian multiplied by $r^2$ where $r$ is the electron-ion distance.

### F. Variational and lattice-regularized diffusion Monte Carlo (VMC, LR-DMC)

#### 1. *Approach and computational details*

In this work we used standard quantum Monte Carlo (QMC) methods by means of correlated variational wave functions defined in real space configurations $x$ where the electrons have definite positions $\vec{r}_{1,\sigma_1}, \vec{r}_{2,\sigma_2} \cdot \vec{r}_{N,\sigma_N}$ and spins $\sigma_i \pm 1/2$ along the $z-$ quantization axis, where $N$ is the number of electrons. The many body wave function is obtained by applying a positive function $J(x)$ symmetric under particle permutations to a Slater Determinant $D(x)$ , antisymmetric under particle permutations:

$$\Psi_T(x) = J(x)D(x) \tag{28}$$

thus satisfying Pauli's principle. Both the Jastrow $J(x)$ and the determinantal $D(x)$ parts are expanded in localized basis sets as described in details in Ref.47.

The determinant part $D(x)$ is obtained by a DFT calculation using modified ccpVDZ and ccpVTZ basis sets. In the standard ccpVTZ we remove he largest $Z_{1s}$ ($Z_{1s} = 33.87$) exponent and the corresponding contraction because the cusp conditions have been fulfilled by a one body Jastrow factor of the type:

$$u_{1-body}(r) = -\frac{1 - \exp(-br)}{b}. \tag{29}$$

This one body Jastrow is included also in the GTO basis set for the DFT (LDA) calculation, where $b = \sqrt{2}$, whereas $b$ is optimized by minimizing the energy in the VMC calculation. The DFT is also defined (within the TurboRVB package[48]) on a mesh of lattice space $a_{DFT} = 0.1$ or smaller, until convergence is reached within $0.001H$ in the total energy. The use of the one body Jastrow factor drastically improves the convergence for $a_{DFT} \to 0$. Within the DFT calculation, satisfying the cusp conditions typically improves the quality of the basis at the level of the ccpVQZ and ccpVTZ, for the ccpVTZ and ccpVDZ ones, respectively. However all these basis sets remain rather poor for small interatomic distances (see Fig. 26). In order to define a simple and compact basis that can be used also in this limit, we have found that it is enough to work with a ccpVDZ basis, again with the largest s-wave exponent ($Z_{1s} = 13.01$) removed, no contraction, and two p-wave gaussians with diffusive exponents $Z_{1p} = 0.2$ and $Z_{2p} = 0.05$. As it is shown in Fig.(26) with this simple receipt, the quality of the basis is satisfactorily accurate (with error less than 1mH/atom) in all the range studied. Similar results can be obtained with standard augmented basis sets with triple or quadruple zeta dimensions, but they are certainly computationally much more demanding for QMC. For clarity all the basis sets used in this work are summarized in Tab. V:

Within periodic boundary conditions in the direction of the chain, assumed to be along the $z$ direction, we use a supercell of dimension $L_x \times L_x \times L_z$ with $L_x = L_y = 40a.u.$, that is large enough for safely neglecting the interaction between the periodic images in the $x, y$ directions (error less than $0.0001H$ per atom). Moreover the basis set (standard for open systems) has been periodized according to the standard procedure described in Ref.49, when PBC are applied.

For the VMC calculation, the trial function $\Psi_T$ contains the so called two (electron-electron), three (electron-electron-ion) and four bodies (electron-electron-ion-ion) contributions that are expanded in a localized basis different from the determinant one. Indeed, in this case, we have used a fully uncontracted basis with the exponents given in the last raw of Tab. V. All the corresponding variational parameters (about 1000 for the largest systems), determining the Jastrow factor $J(x)$ are efficiently optimized, using the scheme described in Ref.50. Since the Jastrow is not affecting the results for $a \to 0$ presented here, we do not describe in details its form and the standard optimization methods used[51].

Once the correlated VMC wave function has been prepared with the optimal choice of $J(x)$, we compute the so called fixed node energies, by employing a more accurate QMC technique, dubbed LR-DMC, briefly described in the following.

The LR-DMC is a projection method[52] that uses the lattice regularization for applying the imaginary time propagator $\exp(-\beta H)$ to a trial function $\Psi_T$ defined in the continuous space. The main approximation is to write the laplacian by means of its dicretized expression on a lattice with a grid with lattice space $a$, e.g. for a single electron wave function depending only

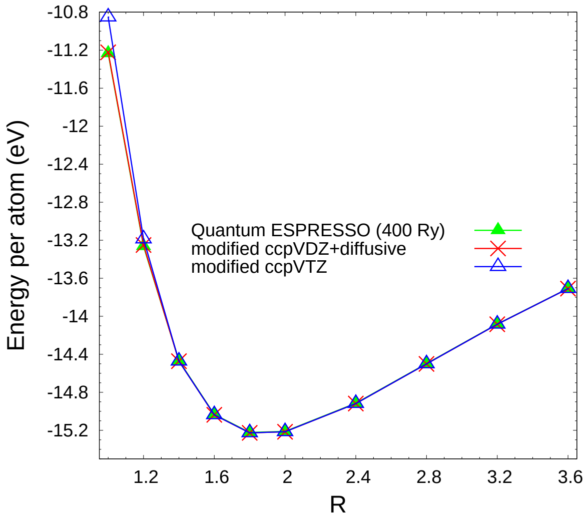


FIG. 26. (color online) Validation of the basis set used for the DFT-LDA calculation. Within TurboRVB it is possible to use exactly the same basis for QMC and DFT (LDA) calculations. Here the DFT energy is compared with the widely used Quantum ESPRESSO plane-wave DFT code[4] for large enough cutoff. By extending the standard ccpVDZ basis with diffusive p orbitals (see text and Tab. V) it is possible to reach a satisfactory accuracy even at small $R$, much better than the ccpVTZ one, even when considering the improvement described in the text and verified in Ref.[47] for the $Na_2$ molecule. Indeed without including diffusive p-orbitals, all any standard basis set with no augmentation (i.e. without diffusive orbitals, containing gaussians with small exponents) becomes quite poor for the Hydrogen chain system in the small $R$ limit.

on one variable $x$: $\nabla\Psi = \partial_x^2\Psi \to \nabla_a\Psi = \frac{1}{a^2}(\Psi(x+a)+\Psi(x-a)-2\Psi(x))$. The extension of $\nabla_a$ to higher dimensions is straightforward and the continuous space can be sampled ergodically even for finite $a > 0$ with a much simpler algorithm than the original proposal[52], namely by randomizing the directions along which the laplacian is discretized[53]. For $a \to 0$ and $\beta \to \infty$ the exact ground state wave function $\Psi_G$ can be obtained if $\langle \Psi_T | \Psi_G \rangle \neq 0$. However, due to the "fermion sign problem", an approximation is employed to achieve small and controlled statistical errors: it is required that, during the projection, the "sign" of the propagated wave function is constrained to the one of the chosen trial function:

$$\Psi_T(x) \times \langle x | \exp(-\beta H) | \Psi_T \rangle \geq 0 \tag{30}$$

for any electronic configuration $x$. For $a \to 0$ the results coincide with the standard Fixed-Node approximation introduced long time ago[54]. This scheme is usually employed within the diffusion short time ($\Delta$) approximation of the propagator, in a way that in the $\Delta \to 0$ limit, by applying it $\frac{\beta}{\Delta}$ times, the exact Fixed node projection scheme (30) is recovered, with the well established variational property on the estimated energy. In this work we have used the lattice regularization, just because it is more conveniently implemented in the TurboRVB package[48], and also because the extrapolations for $a \to 0$ are very well behaved and easily controlled in an automatic way.

Since with QMC calculations we extract electronic configurations in real space, it is particularly easy to calculate the correlation functions. Among the ones employed for this study, certainly a crucial role has been played by the Resta-Sorella phase

$$Z_N = \langle \Psi_N | e^{i\frac{2\pi}{L}\sum_i \hat{x}_i} | \Psi_N \rangle, \tag{31}$$

where $N$ is the number of atoms in the supercell of length $L$. $Z_N$ is a measure of the electron localization[55], yielding the metallic or insulating character of the ground state in a simple and direct way. As we have explained in the paper, for a perfect crystalline structure, $Z_N$ saturated to one for a perfectly localized state for $N \to \infty$, while it vanishes in this limit if there is no localization and the ground state is metallic. In our study we have considered large enough systems to establish that there is no localization when the atoms are close to each other, while the system becomes insulating for larger lattice spacing as it is shown in the paper in Fig. 3b.

*2. Additional data*

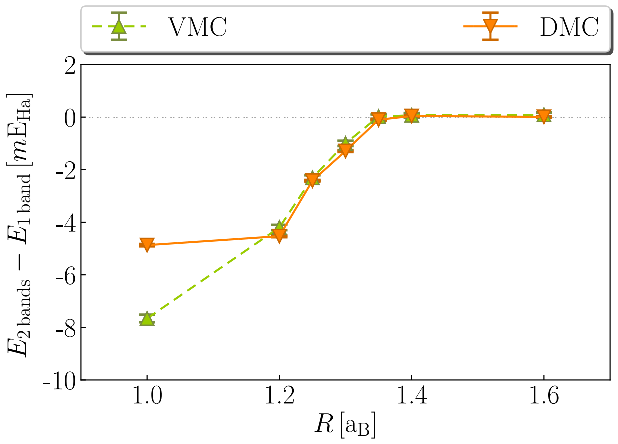


FIG. 27. (color online) VMC (green upward-pointing triangles) and DMC (orange downward-pointing triangles) energy differences as a function of the lattice spacing between the optimal wave functions with no constraints on the occupation of the electronic bands and the wave functions where the occupation of the p-wave bands is not allowed. For $R$ smaller than $R \simeq 1.35 a_B$ the occupancy of the p-wave bands become necessary for the accurate description of the ground state.


[1] R. M. Martin, Electronic Structure: Basic Theory and Practical Methods (Cambridge University Press, 2004).
[2] C. Lin, F. H. Zong, and D. M. Ceperley, Physical Review E **64**, 016702 (2001).
[3] M. Motta, D. M. Ceperley, G. K.-L. Chan, J. A. Gomez, E. Gull, S. Guo, C. A. Jiménez-Hoyos, T. N. Lan, J. Li, F. Ma, A. J. Millis, N. V. Prokof'ev, U. Ray, G. E. Scuseria, S. Sorella, E. M. Stoudenmire, Q. Sun, I. S. Tupitsyn, S. R. White, D. Zgid, and S. Zhang (Simons Collaboration on the Many-Electron Problem), Physical Review X **7**, 031059 (2017).
[4] P. Giannozzi, S. Baroni, N. Bonini, M. Calandra, R. Car, C. Cavazzoni, D. Ceresoli, G. L. Chiarotti, M. Cococcioni, I. Dabo, A. Dal Corso, S. de Gironcoli, S. Fabris, G. Fratesi, R. Gebauer, U. Gerstmann, C. Gougoussis, A. Kokalj, M. Lazzeri, L. Martin-Samos, N. Marzari, F. Mauri, R. Mazzarello, S. Paolini, A. Pasquarello, L. Paulatto, C. Sbraccia, S. Scandolo, G. Sclauzero, A. P. Seitsonen, A. Smogunov, P. Umari, and R. M. Wentzcovitch, Journal of Physics: Condensed Matter **21**, 395502 (19pp) (2009).
[5] J. P. Perdew, K. Burke, and M. Ernzerhof, Phys. Rev. Lett. **77**, 3865 (1996).
[6] D. R. Hamann, Phys. Rev. B **88**, 085117 (2013).
[7] D. R. Hamann, Phys. Rev. B **95**, 239906 (2017).
[8] J. P. Perdew and A. Zunger, Phys. Rev. B **23**, 5048 (1981).
[9] J. Heyd, G. E. Scuseria, and M. Ernzerhof, The Journal of Chemical Physics **118**, 8207 (2003), https://doi.org/10.1063/1.1564060.
[10] J. Heyd, G. E. Scuseria, and M. Ernzerhof, The Journal of Chemical Physics **124**, 219906 (2006), https://doi.org/10.1063/1.2204597.
[11] J.-W. Song, K. Yamashita, and K. Hirao, The Journal of Chemical Physics **135**, 071103 (2011), https://doi.org/10.1063/1.3628522.
[12] S. Zhang and H. Krakauer, Physical Review Letters **90**, 136401 (2003).
[13] M. Motta and S. Zhang, WIREs Comput Mol Sci **e1364**, 1 (2018).
[14] R. L. Stratonovich, Soviet Physics Doklady **2**, 416 (1957).
[15] J. Hubbard, Physical Review Letters **3**, 77 (1959).
[16] J. P. F. LeBlanc, A. E. Antipov, F. Becca, I. W. Bulik, G. K.-L. Chan, C.-M. Chung, Y. Deng, M. Ferrero, T. M. Henderson, C. A. Jiménez-Hoyos, E. Kozik, X.-W. Liu, A. J. Millis, N. V. Prokof'ev, M. Qin, G. E. Scuseria, H. Shi, B. V. Svistunov, L. F. Tocchio, I. S. Tupitsyn, S. R. White, S. Zhang, B.-X. Zheng, Z. Zhu, and E. Gull (Simons Collaboration on the Many-Electron Problem), Physical Review X **5**, 041041 (2015).
[17] M. Qin, H. Shi, and S. Zhang, Physical Review B **94**, 235119 (2016).
[18] B.-X. Zheng, C.-M. Chung, P. Corboz, G. Ehlers, M.-P. Qin, R. M. Noack, H. Shi, S. R. White, S. Zhang, and G. K.-L. Chan (Simons Collaboration on the Many-Electron Problem), Science **358**, 1155 (2017).
[19] F. Ma, S. Zhang, and H. Krakauer, Physical Review B **95**, 165103 (2017).
[20] F. Ma, W. Purwanto, S. Zhang, and H. Krakauer, Physical Review Letters **114**, 226401 (2015).
[21] W. Purwanto, H. Krakauer, Y. Virgus, and S. Zhang, The Journal of Chemical Physics **135**, 164105 (2011).
[22] S. Zhang, J. Carlson, and J. E. Gubernatis, Physical Review B **55**, 7464 (1997).
[23] W. Purwanto and S. Zhang, Phys. Rev. E **70**, 056702 (2004).
[24] M. Motta and S. Zhang, Journal of Chemical Theory and Computation **13**, 5367 (2017), pMID: 29053270.
[25] M. Kalos, Journal of Computational Physics **1**, 257 (1966).
[26] K. S. Liu, M. H. Kalos, and G. V. Chester, Phys. Rev. A **10**, 303 (1974).

[27] W. Purwanto, S. Zhang, and H. Krakauer, Journal of Chemical Theory and Computation **9**, 4825 (2013), pMID: 26583401.
[28] M. Suewattana, W. Purwanto, S. Zhang, H. Krakauer, and E. J. Walter, Physical Review B **75**, 245123 (2007).
[29] M. Motta, S. Zhang, and G. K.-L. Chan, Phys. Rev. B **100**, 045127 (2019).
[30] R. Blankenbecler, D. J. Scalapino, and R. L. Sugar, Phys. Rev. D **24**, 2278 (1981).
[31] S. R. White, D. J. Scalapino, R. L. Sugar, E. Y. Loh, J. E. Gubernatis, and R. T. Scalettar, Phys. Rev. B **40**, 506 (1989).
[32] H. Shi, S. Chiesa, and S. Zhang, Phys. Rev. A **92**, 033603 (2015).
[33] R. A. Kendall, T. H. Dunning Jr, and R. J. Harrison, J. Chem. Phys. **96**, 6796 (1992).
[34] J. McClain, Q. Sun, G. K.-L. Chan, and T. C. Berkelbach, Journal of Chemical Theory and Computation **13**, 1209 (2017), pMID: 28218843.
[35] Q. Sun, T. C. Berkelbach, N. S. Blunt, G. H. Booth, S. Guo, Z. Li, J. Liu, J. D. McClain, E. R. Sayfutyarova, S. Sharma, S. Wouters, and G. K.-L. Chan, WIREs Comput. Mol. Sci. **8**, e1340 (2018).
[36] S. R. White and E. M. Stoudenmire, Phys. Rev. B **99**, 081110 (2019).
[37] S. R. White, Phys. Rev. Lett. **69**, 2863 (1992).
[38] S. R. White, Phys. Rev. B **48**, 10345 (1993).
[39] G. K.-L. Chan, A. Keselman, N. Nakatani, Z. Li, and S. R. White, J. Chem. Phys. **145**, 014102 (2016).
[40] R. Olivares-Amaya, W. Hu, N. Nakatani, S. Sharma, J. Yang, and G. K.-L. Chan, J. Chem. Phys. **142**, 034102 (2015).
[41] C. Edmiston and K. Ruedenberg, Rev. Mod. Phys. **35**, 457 (1963).
[42] G. K.-L. Chan and M. Head-Gordon, J. Chem. Phys. **116**, 4462 (2002).
[43] G. K.-L. Chan, J. Chem. Phys. **120**, 3172 (2004).
[44] G. K.-L. Chan and S. Sharma, Annu. Rev. Phys. Chem. **62**, 465 (2011).
[45] S. Sharma and G. K.-L. Chan, J. Chem. Phys. **136**, 124121 (2012).
[46] E. M. Stoudenmire and S. R. White, Physical Review Letters **119**, 046401 (2017).
[47] K. Nakano, R. Maezono, and S. Sorella, Journal of Chemical Theory and Computation **15**, 4044 (2019), pMID: 31117480, https://doi.org/10.1021/acs.jctc.9b00295.
[48] S. Sorella, "TurboRVB quantum Monte Carlo package," .
[49] R. Dovesi, R. Orlando, A. Erba, C. M. Zicovich-Wilson, B. Civalleri, S. Casassa, L. Maschio, M. Ferrabone, M. D. L. Pierre, P. D'Arco, Y. Noel, M. Causa, M. Rerat, and B. Kirtman, International Journal of Quantum Chemistry **114**, 1287 (2014).
[50] A. Zen, Y. Luo, S. Sorella, and L. Guidoni, Journal of Chemical Theory and Computation **9**, 4332 (2013).
[51] M. Marchi, S. Azadi, M. Casula, and S. Sorella, The Journal of Chemical Physics **131**, 154116 (2009).
[52] M. Casula, C. Filippi, and S. Sorella, Physical Review Lettersrs **95**, 100201 (2005).
[53] M. Casula, S. Moroni, S. Sorella, and C. Filippi, The Journal of Chemical Physics **132**, 154113 (2010).
[54] P. Reynolds, D. Ceperley, B. Alder, and J. Lester, The Journal of Chemical Physics **77**, 5593 (1982).
[55] R. Resta and S. Sorella, Physical Review Letters **82**, 370 (1999).
